# Supplementary material for: Kitaev physics in the two-dimensional magnet NiPSe$_3$
Source: arXiv:2403.09831 source file (2024-03-14)
Supplement: Supplementary file 1 [file supplementary_material.pdf]

# Supplmentary Materials:
# Kitaev physics in the two-dimensional magnet $NiPSe_3$


Cheng Peng,[1,*] Sougata Mardanya,[2,†] Alexander Petsch,[1,3] Vineet Kumar Sharma,[2]
Shuyi Li,[4] Chunjing Jia,[4] Arun Bansil,[5] Sugata Chowdhury,[2] and Joshua J. Turner[1,3,‡]

[1] *Stanford Institute for Materials and Energy Sciences, Stanford University, Menlo Park, CA, USA*
[2] *Department of Physics and Astronomy, Howard University, Washington DC, USA*
[3] *Linac Coherent Light Source, SLAC National Accelerator Laboratory, Menlo Park, CA, USA*
[4] *Department of Physics, University of Florida, Gainesville, Florida 32611, USA*
[5] *Department of Physics, Northeastern University, Boston, Massachusetts 02115, USA*



(Dated: March 14, 2024)


## I. NUMERICAL METHODS

We have performed first-principles calculations within the framework of the density-functional theory (DFT) [1] using the Vienna *ab-initio* simulation package (VASP) [2, 3]. The ground-state electronic structure is obtained with the projector-augmented-wave pseudo-potential, while the electron exchange-correlation effects are treated via the generalized gradient approximation (GGA) [4] with Perdew-Burke-Ernzerhof (PBE) parametrization. The strong correlation effects in the valance Ni-$d$ orbitals are corrected through an effective onsite Hubbard potential ($U_{\text{eff}}$) [5, 6]. All calculations are based on $U_{\text{eff}} = 4.0$ eV. The weak interlayer-vdW interaction is treated by the DFT-D3 correction of Grimme with zero-damping function [7]. An energy cut-off of 350 eV was utilized for the plane-wave basis set, and the Brillouin zone (BZ) integration was performed over an $11\times9\times11$ $\Gamma$-centered $k$-mesh [8]. The total-energy tolerance criterion is set at $10^{-5}$ eV in the self-consistency cycles. Starting with the experimental structure we optimized both the cell parameters and the ionic positions until the residual forces on each ion were below $10^{-2}$ eV/Å and the stress tensors became negligible. We used the single-particle Green's function with rigid spin rotation as perturbation, following Liechtenstein, Katsnelson, Antropov, and Gubanov (LKAG) [9], which is implemented in the TB2J code [10]. To obtain the single-particle Green's function, we constructed a low-energy tight-binding model Hamiltonian from the atom-centered Wannier functions using the Ni $d$ and $s$-$p$ orbitals in the Wannier90 code suite [11]. Effects of spin-orbit coupling (SOC) are incorporated in the projected-augmented wave (PAW) method in VASP as the perturbed Hamiltonian $H_{SO}^{\alpha\beta} = -\frac{\hbar^2}{(2m_ec)^2}\frac{K(r)}{r}\frac{dV(\vec{r})}{dr}\boldsymbol{\sigma}^{\alpha\beta}\cdot\mathbf{L}$ [12], where $\mathbf{L}$ is the orbital moment operator, $\boldsymbol{\sigma}$ are the Pauli spin matrices, $V(r)$ is the spherical part of the PAW potential and $K(r)$ is defined as $(1 - V(\vec{r})/2m_ec^2)^{-2}$. To tune the SOC strength, we revised the pre-factor of the $\boldsymbol{\sigma}\cdot\mathbf{L}$ term in the VASP source code.

## II. KEY ASPECTS OF MATERIALS UNDER STUDY

$NiPS_3$ and $NiPSe_3$ are both Mott insulators [13–15]. In $NiPS_3$, through fitting of the neutron scattering data using the corresponding theoretical results based on the linear spin-wave theory, it is found that the nearest-neighbor spin coupling is *ferromagnetic* [16, 17]. This implies that the spin coupling in $NiPS_3$ predominantly results from superexchange, i.e. via electron hopping through the Sulfur $p$-orbitals [18], because the direct exchange between the two neighboring Ni sites, without involving any ligands, will yield *antiferromagnetic* spin interactions. According to earlier numerical studies [19–22], the Heisenberg spin interactions between the first-, second- and third-nearest-neighbor Ni sites within a single honeycomb layer, as described in Fig. 1b in the main text remain qualitatively the same in bulk for $NiPSe_3$. However, Se has a larger ionic radius and stronger SOC in its $3p$ orbitals than S, which alters the hopping integrals for overlapping orbitals and the charge transfer gap between the Ni ions and the Se ligands. More importantly, previous DFT results show that Ni in a $3d^8$ configuration has fully occupied $t_{2g}$ orbitals, which leave the $e_g$ orbitals half-filled, and yield via the Hund's coupling a favored spin configuration of $S = 1$ [14]. Band structure calculations show that the $e_g$ orbitals are strongly hybridized with the surrounding octahedra of S/Se $p$-orbitals [20]. Our calculations confirm the properties summarized above in this paragraph, we illustrate these results through the orbital-projected band structure and density of state calculations in Fig. S1.


[*] These authors contributed equally to this work.; cpeng18@stanford.edu
[†] These authors contributed equally to this work.
[‡] joshuat@slac.stanford.edu

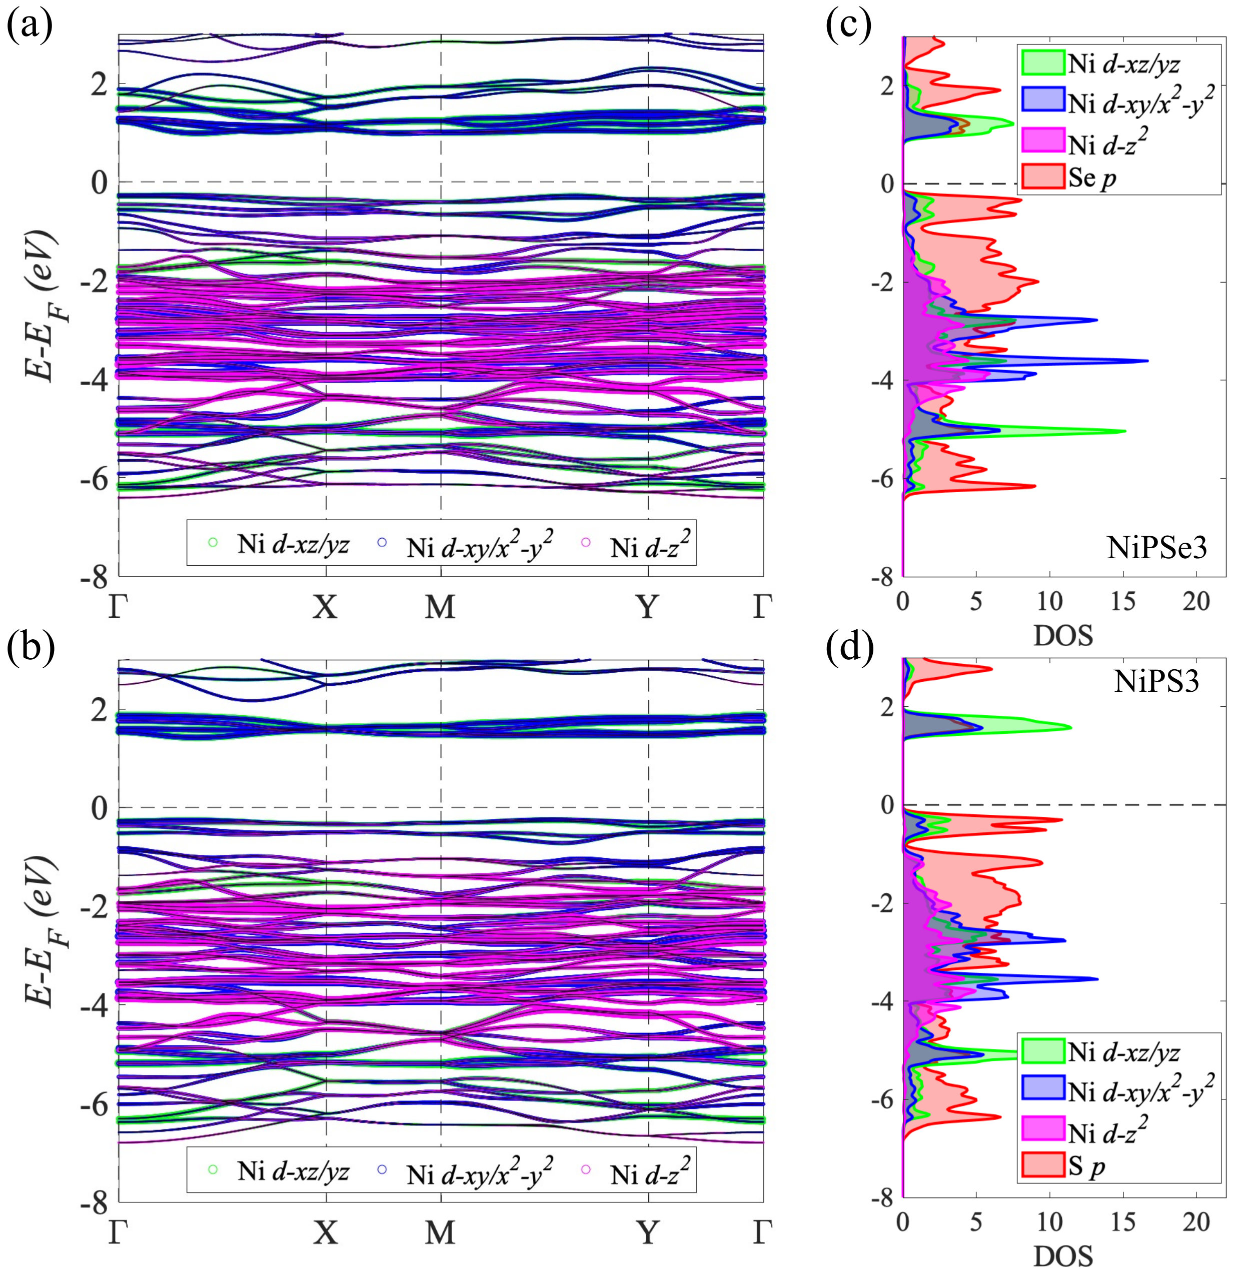


FIG. S1. Orbital-projected electronic structure of (a) $NiPSe_3$ and (b) $NiPS_3$, along high-symmetry paths in the Brillouin zone, respectively. Different colors represent various orbital while the marker size is proportional to the orbital weight. Local density of state for (c) $NiPSe_3$ and (d) $NiPS_3$.

$NiPSe_3$ crystallizes in the space group $C2/m$ (#12) with four Ni atoms at the 4g Wyckoff position, four P atoms at the 4i Wyckoff position, and four $Se_1$ and eight $Se_2$ atoms at the 4i and 8j Wyckoff positions, respectively. The lattice parameters for the conventional unit cell are a=6.14396 Å, b=10.65457 Å, and c=6.92586 Å, where a and b are orthogonal to each other and c is tilted by 16.73° with respect to the normal to the ab-plane. For a better understanding of the hopping amplitude between the Ni-$d$ and Se-$p$ orbitals, we consider rotating the Wannier orbitals along the bond directions of the octahedra surrounding the Ni atoms, as depicted in Fig. 1c of the main text.

Table S1 gives values of $J_1$ to $J_4$, with $J_1$ to $J_3$ representing the first-, second-, and third-nearest-neighbor spin interactions in the hexagonal lattice of Ni, and $J_4$ denoting the inter-layer coupling. Note that the single-ion anisotropy is non-negligible in $NiPX_3$ ($X$ = {S, Se}) [17, 23, 24]. We have not computed single-ion anisotropies, which are considered beyond the scope of our study.

| | $J_1$ | $J_2$ | $J_3$ | $J_4$ | $K^{\gamma}$ |
|---|---|---|---|---|---|
| $NiPS_3$ | 2.4852 | 0.0828 | −9.4798 | 0.0196 | −0.001 |
| $NiPSe_3$ | 1.304 | 0.0628 | −12.766 | 0.0204 | 0.0608 |
| *$NiPSe_3$ | 1.493 | 0.1974 | −12.727 | 0.0266 | 0.2434 |

TABLE S1. Magnetic coupling constants (in meV) computed using the TB2J software [10] for Ni$PX_3$ ($X = \{\text{S, Se}\}$). A negative $J_3$ value indicates that the third-nearest-neighbor superexchange is *antiferromagnetic*. Note that TB2J does not allow the computation of single-ion anisotropy, which is minor but critically important for stabilizing the magnetic order [17, 23, 24].

## III. DERIVATION OF PERTURBATION THEORY

Magnetic properties of the transition-metal chalcogenophosphates $M\mathrm{P}X_3$ ($M = \{\text{Mn, Fe, Ni}\}$) can be described theoretically via effective spin models that range from large to small spins involving on-site Kanamori interaction combined with tight-binding Hamiltonians for orbitals of neighboring atoms as a perturbation to the on-site Hamiltonian.

We refer to the derivation via perturbation theory in Refs. [18, 25–32] for modeling spin interactions in a single-layered hexagonal lattice, including SOC for ligand atoms. In our local model, the on-site Hamiltonian includes two magnetic Ni atoms (denoted as $M_1$ and $M_2$) positioned at the centers of the octahedral cages, and two ligand Se atoms (denoted $X_1$ and $X_2$) on the shared edges of the two neighboring octahedral cages. Since the $p$ orbitals are fully occupied, we simplify our approach by considering only a one-hole processes, where each ligand site can host at most one hole at any time. As a result, the SOC leads to the modified on-site Hamiltonian:

$$H_{\mathrm{SOC}} = \lambda_p \mathbf{L}\cdot\mathbf{S} = \lambda_p[\frac{1}{2}(L^+S^- + L^-S^+) + L^zS^z] \tag{1}$$

where, $\lambda_p$ is the strength of SOC, $\mathbf{L}$ is the angular momentum, $\mathbf{S}$ is the spin-$\frac{1}{2}$ operator, which can be decomposed as $S^+ = \begin{pmatrix} 0 & 1 \\ 0 & 0 \end{pmatrix}$, $S^- = \begin{pmatrix} 0 & 0 \\ 1 & 0 \end{pmatrix}$, and $S^z = \frac{1}{2}\begin{pmatrix} 1 & 0 \\ 0 & -1 \end{pmatrix}$, where $c = \hbar = 1$. The real spherical harmonics for the $p$ atomic orbital with $l = 1$ satisfy the following relations, where the arguments $(\theta, \phi)$ of the $Y_l^m$ have been omitted for simplicity,

$$\begin{aligned} Y_{1,1} =& |p_x\rangle = \frac{1}{\sqrt{2}}(Y_1^{-1} - Y_1^1) \\ Y_{1,-1} =& |p_y\rangle = \frac{i}{\sqrt{2}}(Y_1^{-1} + Y_1^1) \\ Y_{1,0} =& |p_z\rangle = Y_1^0 \end{aligned}$$

Recall the operations of operators on the real spherical harmonics, *i.e.* $L_\pm Y_l^m = \sqrt{(l \mp m)(l \pm m + 1)}Y_l^{m\pm 1}$ and $L_z Y_l^m = mY_l^m$, from which one obtains for the matrix representation of $L_+$, $L_-$ and $L_z$ in $\{|p_x\rangle, |p_y\rangle, |p_z\rangle\}$ basis:

$$\begin{aligned} L_+|p_x\rangle =& L_+\frac{1}{\sqrt{2}}(Y_1^{-1} - Y_1^1) = Y_1^0 = |p_z\rangle \\ L_+|p_y\rangle =& L_+\frac{i}{\sqrt{2}}(Y_1^{-1} + Y_1^1) = iY_1^0 = i|p_z\rangle \\ L_+|p_z\rangle =& L_+Y_1^0 = \sqrt{2}Y_1^1 = -i|p_y\rangle - |p_x\rangle \\ L_z|p_x\rangle =& L_z\frac{1}{\sqrt{2}}(Y_1^{-1} - Y_1^1) = -\frac{1}{\sqrt{2}}(Y_1^{-1} + Y_1^1) = i|p_y\rangle \\ L_z|p_y\rangle =& L_z\frac{i}{\sqrt{2}}(Y_1^{-1} + Y_1^1) = -\frac{i}{\sqrt{2}}(Y_1^{-1} - Y_1^1) = -i|p_x\rangle \\ L_z|p_z\rangle =& L_zY_1^0 = 0 \end{aligned}$$

Then one obtains $L^+ = \begin{pmatrix} 0 & 0 & -1 \\ 0 & 0 & -i \\ 1 & i & 0 \end{pmatrix}$ and $L^- = \begin{pmatrix} 0 & 0 & 1 \\ 0 & 0 & -i \\ -1 & i & 0 \end{pmatrix}$. Considering spin yields

$$\begin{aligned} L_+S_-|p_{x\uparrow}\rangle =&|p_{z\downarrow}\rangle \\ L_+S_-|p_{x\downarrow}\rangle =&0 \\ L_+S_-|p_{y\uparrow}\rangle =&i|p_{z\downarrow}\rangle \\ L_+S_-|p_{y\downarrow}\rangle =&0 \\ L_+S_-|p_{z\uparrow}\rangle =&-i|p_{y\downarrow}\rangle - |p_{x\downarrow}\rangle \\ L_+S_-|p_{z\downarrow}\rangle =&0 \end{aligned}$$

In the $\{|p_{x\uparrow}\rangle, |p_{x\downarrow}\rangle, |p_{y\uparrow}\rangle, |p_{y\downarrow}\rangle, |p_{z\uparrow}\rangle, |p_{z\downarrow}\rangle\}$ basis, the matrices are represented as $L^+S^- = \begin{pmatrix} 0 & 0 & 0 & 0 & 0 & 0 \\ 0 & 0 & 0 & 0 & -1 & 0 \\ 0 & 0 & 0 & 0 & 0 & 0 \\ 0 & 0 & 0 & 0 & -i & 0 \\ 0 & 0 & 0 & 0 & 0 & 0 \\ 1 & 0 & i & 0 & 0 & 0 \end{pmatrix}$,

$L^-S^+ = \begin{pmatrix} 0 & 0 & 0 & 0 & 0 & 1 \\ 0 & 0 & 0 & 0 & 0 & 0 \\ 0 & 0 & 0 & 0 & 0 & -i \\ 0 & 0 & 0 & 0 & 0 & 0 \\ 0 & -1 & 0 & i & 0 & 0 \\ 0 & 0 & 0 & 0 & 0 & 0 \end{pmatrix}$ and $L^zS^z = \frac{i}{2}\begin{pmatrix} 0 & 0 & -1 & 0 & 0 & 0 \\ 0 & 0 & 0 & 1 & 0 & 0 \\ 1 & 0 & 0 & 0 & 0 & 0 \\ 0 & -1 & 0 & 0 & 0 & 0 \\ 0 & 0 & 0 & 0 & 0 & 0 \\ 0 & 0 & 0 & 0 & 0 & 0 \end{pmatrix}$.

Substituting back into Eq.1 gives the matrix representation of $H_{\rm SOC}$ as:

$$\begin{aligned} H_{\rm SOC} =&\lambda_p[\frac{1}{2}(L^+S^- + L^-S^+) + L^zS^z] \\ =&\frac{i}{2}\lambda_p \begin{pmatrix} 0 & 0 & -1 & 0 & 0 & -i \\ 0 & 0 & 0 & 1 & i & 0 \\ 1 & 0 & 0 & 0 & 0 & -1 \\ 0 & -1 & 0 & 0 & -1 & 0 \\ 0 & i & 0 & 1 & 0 & 0 \\ -i & 0 & 1 & 0 & 0 & 0 \end{pmatrix} \\ =&i\lambda_p \begin{pmatrix} \mathbf{0}_{2\times2} & -S^z & S^y \\ S^z & \mathbf{0}_{2\times2} & -S^x \\ -S^y & S^x & \mathbf{0}_{2\times2} \end{pmatrix} \end{aligned}$$

where $S^x$, $S^y$, and $S^z$ are the spin operator matrices for spin-$\frac{1}{2}$, and $\mathbf{0}_{2\times2}$ is the $2\times2$ zero matrix. The eigenvalues of $H_{\rm SOC}$ are $\{-\lambda_p, -\lambda_p, \frac{\lambda_p}{2}, \frac{\lambda_p}{2}, \frac{\lambda_p}{2}, \frac{\lambda_p}{2}\}$. Referring to Ref. [26], the nonmagnetic ligand (X) sites, with fully occupied $p$ orbitals $\{p_x, p_y, p_z\}$, mediate the superexchange of electrons (holes) between the magnetic atoms. In the magnetic sites (M), the $e_g$ orbitals are half-filled. For the ligand mediated superexchange, it is more straightforward to consider holes rather than electrons. We focus on the two possible hopping paths presented by single-hole processes in which the excited states involve the movement of hole from one of the Ni $e_g$ orbitals to one of the three $p$ orbitals of the ligand. It is necessary to consider the SOC of $p$ orbitals through a perturbative procedure (truncated at second order) to calculate the indirect $d$-to-$d$ hopping integrals. Following Ref. [28], the intermediate state has the energy $\Delta E_h = \varepsilon_d - \varepsilon_p - \lambda_p$ or $\varepsilon_d - \varepsilon_p + \frac{\lambda_p}{2}$, with $\varepsilon_d$ and $\varepsilon_p$ representing the atomic energy difference between $M$ and $X$ sites, respectively. Similar to Eq.(3) of Ref. [28], the tight-binding model with effective hoppings between the nearest-neighbor Ni atoms takes the form:

$$T_{12}^{\rm eff} + T_{12}^{\rm eff\dagger} = d_{M_1}^\dagger T_{M_1M_2}^{\rm eff} d_{M_2} + {\rm H.C.} \tag{2}$$

Here, the creation operators $d_{M_m}^\dagger = (d_{M_m,x^2-y^2\uparrow}^\dagger,\ d_{M_m,x^2-y^2\downarrow}^\dagger,\ d_{M_m,z^2\uparrow}^\dagger,\ d_{M_m,z^2\downarrow}^\dagger)$ create one hole with spin in one of the $e_g$ orbitals of $M_m (m = 1, 2)$. The general hopping matrix for the indirect $d$-to-$d$ hopping is generally defined as

$$T_{M_1M_2}^{\rm eff} = \sum_{m=1,2} T_{M_1X_m} \sum_h \frac{|h\rangle\langle h|}{\Delta E_h} T_{X_mM_2} = \sum_{m=1,2} T_{M_1X_m}(\Delta_{pd}\mathbf{I} + H_{\rm SOC})^{-1} T_{X_mM_2} \tag{3}$$

where the sum is over all single-hole states $|h\rangle$ of the site $X_m$, along with a sum over the related ligand site $m$ that mediates the super-exchange between a pair of nearest-neighbor Ni atoms. $\sum_h \frac{|h\rangle\langle h|}{\Delta E_h}$ can equivalently rewritten as:

$$(\Delta_{pd}\mathbf{I} + H_{\mathrm{SOC}})^{-1} = \begin{pmatrix} \alpha\mathbf{I} & \beta(-iS^z) & \beta(iS^y) \\ \beta(iS^z) & \alpha\mathbf{I} & \beta(-iS^x) \\ \beta(-iS^y) & \beta(iS^x) & \alpha\mathbf{I} \end{pmatrix} \tag{4}$$

This matrix is given in the basis of $p_{X_m} = (p_{X_m,x\uparrow},\ p_{X_m,x\downarrow},\ p_{X_m,y\uparrow},\ p_{X_m,y\downarrow},\ p_{X_m,z\uparrow},\ p_{X_m z\downarrow})^T$ basis set, where $\mathbf{I}$ is the $2\times 2$ identity matrix, $\alpha = \frac{1}{3}(\frac{1}{\Delta_{pd}-\lambda_p} + \frac{2}{\Delta_{pd}+\frac{\lambda_p}{2}})$ and $\beta = \frac{-\alpha\lambda_p}{2\Delta_{pd}-\lambda_p}$, and $\Delta_{pd} = \varepsilon_d - \varepsilon_p$

Now we consider holes rather than electrons, and consider the same edge-shared octahedra of the honeycomb unit cell in the global coordinates $\{x, y, z\}$ shown in Fig. 1 of Ref. [28] except that for $3d^8$ systems one needs to consider $e_g$ orbitals rather than $t_{2g}$ orbitals; we also need to consider the hopping matrix for the $p$ to $d$ hopping of a hole, as shown in TABLE II of Ref. [26]. The single-hole process of tight-binding model for one hole hopping from $M_2$ to $M_1$ through $X_1$ and $X_2$, *e.g.*, $(M_1 \Leftarrow X_1 \Leftarrow M_2) + (M_1 \Leftarrow X_2 \Leftarrow M_2)$, then is:

$$\begin{aligned} T_{12}^{\mathrm{eff}} =& d_{M_1}^{\dagger} \begin{pmatrix} t_1\mathbf{I} & \mathbf{0} & \mathbf{0} \\ -t_2\mathbf{I} & \mathbf{0} & \mathbf{0} \end{pmatrix} \begin{pmatrix} \alpha\mathbf{I} & \beta(-iS^z) & \beta(iS^y) \\ \beta(iS^z) & \alpha\mathbf{I} & \beta(-iS^x) \\ \beta(-iS^y) & \beta(iS^x) & \alpha\mathbf{I} \end{pmatrix} \begin{pmatrix} \mathbf{0} & \mathbf{0} \\ -t_1\mathbf{I} & -t_2\mathbf{I} \\ \mathbf{0} & \mathbf{0} \end{pmatrix} d_{M_2} \\ &+ d_{M_1}^{\dagger} \begin{pmatrix} \mathbf{0} & t_1\mathbf{I} & \mathbf{0} \\ \mathbf{0} & t_2\mathbf{I} & \mathbf{0} \end{pmatrix} \begin{pmatrix} \alpha\mathbf{I} & \beta(-iS^z) & \beta(iS^y) \\ \beta(iS^z) & \alpha\mathbf{I} & \beta(-iS^x) \\ \beta(-iS^y) & \beta(iS^x) & \alpha\mathbf{I} \end{pmatrix} \begin{pmatrix} -t_1\mathbf{I} & t_2\mathbf{I} \\ \mathbf{0} & \mathbf{0} \\ \mathbf{0} & \mathbf{0} \end{pmatrix} d_{M_2} \\ =& d_{M_1}^{\dagger} \begin{pmatrix} \mathbf{0} & 2t_1t_2\beta(iS^z) \\ -2t_1t_2\beta(iS^z) & \mathbf{0} \end{pmatrix} d_{M_2} \end{aligned}$$

Here, for simplicity, we have used $\mathbf{0}$ to represent the $2\times 2$ zero matrix, and $\mathbf{I}$ is identity.

Our focus in this study is on systems that preserve perfect cubic symmetry in edge-sharing octahedra. However, the presence of a phosphorus dimer at the center of each hexagonal unit can cause deviations from the perfect octahedral structure. Therefore, we utilize DFT methods to calculate the effective spin interactions in the actual material, taking lattice distortions into account. Effects of lattice distortion in $CrI_3$ have been discussed in Ref. [28]. We expect the main physics to be insensitive to effects of gentle lattice distortions, and for this reason, we will focus on the simpler analytical approach and resort to numerical methods for addressing the more complex and realistic scenarios.

Treating $T_{12}^{\mathrm{eff}} + T_{12}^{\mathrm{eff}\dagger}$ as a perturbation to the on-site Hamiltonian containing $M_1, M_2, X_1, X_2$, an effective Hamiltonian within the $S = 1$ subspace can be constructed along the lines of Eq.(6) in the Supplementary Material of Ref. [27], which reads as

$$H^{\mathrm{eff}} \sim -\sum_{\alpha\beta}\sum_{n\neq 0}(\frac{\langle\alpha|T_{12}^{\mathrm{eff}\dagger}|n\rangle\langle n|T_{12}^{\mathrm{eff}}|\beta\rangle}{E_n - E_0} + \frac{\langle\alpha|T_{12}^{\mathrm{eff}}|n\rangle\langle n|T_{12}^{\mathrm{eff}\dagger}|\beta\rangle}{E_n - E_0})|\alpha\rangle\langle\beta| \tag{5}$$

The first term here corresponds to a single hole hopping in a loop from $M_2$ to $M_1$ and then back to $M_2$; the second term is the conjugate process, reversing $M_1$ and $M_2$ in the first term. The excited states are represented by $|n\rangle$ with energy $E_n$ which is higher than $E_0$. $|\alpha\rangle$ and $|\beta\rangle$ are $S = 1$ states of $M_1$ and $M_2$ of form $|S_{M_1}, S_{M_2}, m_1, m_2\rangle = |1, 1, m_1, m_2\rangle \equiv |m_1, m_2\rangle$. $|m_1, m_2\rangle$ running over the $S = 1$ states, $|-1,-1\rangle$, $|-1,0\rangle$, $|-1,1\rangle$, $|0,-1\rangle$, $|0,0\rangle$, $|0,1\rangle$, $|1,-1\rangle$, $|1,0\rangle$, and $|1,1\rangle$. Since the effective Hamiltonian gives all spin couplings through hopping between $M_1$ and $M_2$, the resulting spin model which contains Kitaev, Heisenberg and off-diagonal interactions is:

$$H^{\mathrm{eff}} = J\ \mathbf{S}_1\cdot\mathbf{S}_2 + K^{\gamma}S_1^{\gamma}S_2^{\gamma} + \Gamma\left(S_1^{\alpha}S_2^{\beta} + S_1^{\beta}S_2^{\alpha}\right) + \Gamma'\left(S_1^{\alpha}S_2^{\gamma} + S_1^{\gamma}S_2^{\alpha} + S_1^{\beta}S_2^{\gamma} + S_1^{\gamma}S_2^{\beta}\right).$$

Here, $J$ represents Heisenberg interactions, which are isotropic across the three coordinates of each site on a single-layer honeycomb lattice. $K^{\gamma}$ denotes the bond-dependent Kitaev interactions on the honeycomb lattice, with $\{\alpha, \beta, \gamma\}$ corresponding to rotations $\{y, z, x\}$, $\{z, x, y\}$, and $\{x, y, z\}$ for the $yz$, $zx$, and $xy$ planes, respectively. The axes $\{x, y, z\}$ are depicted in Fig. 1b of the main text. The symmetric off-diagonal terms $\Gamma$ and $\Gamma'$ are zero when without effect of octahedral distortions are neglected.

For the global coordinates in the $xy$-plane (yellow diamond-shaped area in Fig.1b of the main text), the coefficients $J_{\mathrm{ind}}^z$ and $K^z$ from indirect hopping through the ligands between the edge-sharing octahedra can be determined from the matrix element

$$
\begin{aligned}
J^z_{\text{ind}} =& \langle +1, 0|H^{\text{eff}}|0, +1\rangle \\
K^z =& \langle +1, +1|H^{\text{eff}}|+1, +1\rangle - J^z_{\text{ind}}
\end{aligned}
$$

Note that $J^z_{\text{ind}}$ is ferromagnetic if two distinct $p$ orbitals are involved in the single-hole process, as depicted in Fig. 7 of Ref. [33]. Direct hopping between $M_1$ and $M_2$ may also occur but it is likely to be very weak because $J_1$ is *ferromagnetic*, which can only be explained using the super-exchange through the ligand [18, 33]. The *ferromagnetic* $J_1$ is also supported by our DFT simulations for $NiPSe_3$, which yield results similar to those in the literature [19, 20]. Linear spin wave fitting of the magnetic spectra of $NiPS_3$ [17] also show that the nearest neighbor spin coupling is ferromagnetic. These results suggest that, similar to $NiPS_3$, in $NiPSe_3$ also the ligand-mediated superexchange through the edge-sharing octahedral structure is more significant.

In the following derivation, we will use a matrix notations for simplicity. Because $|0, +1\rangle = |0\rangle_{M_1} \otimes |+1\rangle_{M_2}$ and $|0\rangle_{M_1}$ is the $|S_{M_1} = 1, m_1 = 0\rangle$ state of two spins on $M_1$, the eigenstate is represented by $|0\rangle_{M_1} = \frac{1}{\sqrt{2}}(\frac{\uparrow}{M_1,d_{x^2-y^2}}\frac{\downarrow}{M_1,d_{z^2}} + \frac{\downarrow}{M_1,d_{x^2-y^2}}\frac{\uparrow}{M_1,d_{z^2}})$ for $e_g$ orbitals of $M_1$ and $|+1\rangle_{M_2} = \frac{\uparrow}{M_2,d_{x^2-y^2}}\frac{\uparrow}{M_2,d_{z^2}}$ for $e_g$ orbitals of $M_2$. The formulae with electron creation and annihilation operators for the two states are

$$
\begin{aligned}
|0\rangle_{M_1} &= \frac{1}{2}(d^\dagger_{M_1,x^2-y^2\uparrow}d^\dagger_{M_1,z^2\downarrow} + d^\dagger_{M_1,x^2-y^2\downarrow}d^\dagger_{M_1,z^2\uparrow} - d^\dagger_{M_1,z^2\uparrow}d^\dagger_{M_1,x^2-y^2\downarrow} - d^\dagger_{M_1,z^2\downarrow}d^\dagger_{M_1,x^2-y^2\uparrow})|\text{vac}\rangle_{M_1} \\
|+1\rangle_{M_2} &= \frac{1}{\sqrt{2}}(d^\dagger_{M_2,x^2-y^2\uparrow}d^\dagger_{M_2,z^2\uparrow} - d^\dagger_{M_2,z^2\uparrow}d^\dagger_{M_2,x^2-y^2\uparrow})|\text{vac}\rangle_{M_2},
\end{aligned}
$$

where $|\text{vac}\rangle_{M_1}$ and $|\text{vac}\rangle_{M_2}$ are vacuum states for holes (zero hole) on $M_1$ and $M_2$, respectively. In the form of matrix product, we use a general form to conduct operation on states $|0\rangle_{M_1}$ and $|\pm1\rangle_{M_1}$.

| | $\uparrow\uparrow$ | $\uparrow\downarrow$ | $\downarrow\uparrow$ | $\downarrow\downarrow$ |
|---|---|---|---|---|
| $d^\dagger_{M_1,x^2-y^2\uparrow}$ | $d^\dagger_{M_1,z^2\uparrow}$ | $d^\dagger_{M_1,z^2\downarrow}$ | 0 | 0 |
| $d^\dagger_{M_1,x^2-y^2\downarrow}$ | 0 | 0 | $d^\dagger_{M_1,z^2\uparrow}$ | $d^\dagger_{M_1,z^2\downarrow}$ |
| $d^\dagger_{M_1,z^2\uparrow}$ | $-d^\dagger_{M_1,x^2-y^2\uparrow}$ | 0 | $-d^\dagger_{M_1,x^2-y^2\downarrow}$ | 0 |
| $d^\dagger_{M_1,z^2\downarrow}$ | 0 | $-d^\dagger_{M_1,x^2-y^2\uparrow}$ | 0 | $-d^\dagger_{M_1,x^2-y^2\downarrow}$ |

·

| | $\|+1\rangle_{M_1}$ | $\|0\rangle_{M_1}$ | $\|-1\rangle_{M_1}$ |
|---|---|---|---|
| $\uparrow\uparrow$ | 1 | 0 | 0 |
| $\uparrow\downarrow$ | 0 | $\frac{1}{\sqrt{2}}$ | 0 |
| $\downarrow\uparrow$ | 0 | $\frac{1}{\sqrt{2}}$ | 0 |
| $\downarrow\downarrow$ | 0 | 0 | 1 |

$|\text{vac}\rangle_{M_1}$

For $M_2$ it's the same but only replace $M_1$ with $M_2$ in the matrices. Note that we have neglected the normalization factor of $\frac{1}{\sqrt{2}}$ before the matrix here, but that does not change the scaling of the energy spectrum because the normalization factor is an constant.

$$
\begin{aligned}
&T_{12}^{\text{eff}}|0,+1\rangle \\
=&d^\dagger_{M_1}\begin{pmatrix} d^\dagger_{M_1,z^2\uparrow} & d^\dagger_{M_1,z^2\downarrow} & 0 & 0 \\ 0 & 0 & d^\dagger_{M_1,z^2\uparrow} & d^\dagger_{M_1,z^2\downarrow} \\ -d^\dagger_{M_1,x^2-y^2\uparrow} & 0 & -d^\dagger_{M_1,x^2-y^2\downarrow} & 0 \\ 0 & -d^\dagger_{M_1,x^2-y^2\uparrow} & 0 & -d^\dagger_{M_1,x^2-y^2\downarrow} \end{pmatrix}\begin{pmatrix} 0 \\ \frac{1}{\sqrt{2}} \\ \frac{1}{\sqrt{2}} \\ 0 \end{pmatrix}|\text{vac}\rangle_{M_1} \\
&\otimes d^\dagger_{M_1}\begin{pmatrix} \mathbf{0} & 2t_1t_2\beta(iS^z) \\ -2t_1t_2\beta(iS^z) & \mathbf{0} \end{pmatrix}\begin{pmatrix} d^\dagger_{M_2,z^2\uparrow} & d^\dagger_{M_2,z^2\downarrow} & 0 & 0 \\ 0 & 0 & d^\dagger_{M_2,z^2\uparrow} & d^\dagger_{M_2,z^2\downarrow} \\ -d^\dagger_{M_2,x^2-y^2\uparrow} & 0 & -d^\dagger_{M_2,x^2-y^2\downarrow} & 0 \\ 0 & -d^\dagger_{M_2,x^2-y^2\uparrow} & 0 & -d^\dagger_{M_2,x^2-y^2\downarrow} \end{pmatrix}\begin{pmatrix} 1 \\ 0 \\ 0 \\ 0 \end{pmatrix}|\text{vac}\rangle_{M_2} \\
=&\frac{1}{\sqrt{2}}(d^\dagger_{M_1,x^2-y^2\uparrow}d^\dagger_{M_1,z^2\downarrow}+d^\dagger_{M_1,x^2-y^2\downarrow}d^\dagger_{M_1,z^2\uparrow}-d^\dagger_{M_1,z^2\downarrow}d^\dagger_{M_1,x^2-y^2\uparrow}-d^\dagger_{M_1,z^2\uparrow}d^\dagger_{M_1,x^2-y^2\downarrow})|\text{vac}\rangle_{M_1} \\
&\otimes(-it_1t_2\beta d^\dagger_{M_1,x^2-y^2\uparrow}d^\dagger_{M_2,x^2-y^2\uparrow}-it_1t_2\beta d^\dagger_{M_1,z^2\uparrow}d^\dagger_{M_2,z^2\uparrow})|\text{vac}\rangle_{M_2} \\
=&-i\sqrt{2}t_1t_2\beta\left[\begin{array}{ccccccc} & & \overline{X_1,p_x} & \overline{X_1,p_y} & \overline{X_1,p_z} & & \\ \underset{M_1,d_{x^2-y^2}}{\underline{\uparrow\downarrow}} & \underset{M_1,d_{z^2}}{\underline{\uparrow}} & & & & \underset{M_2,d_{x^2-y^2}}{\underline{\uparrow}} & \underset{M_2,d_{z^2}}{\underline{\quad}} \\ & & \overline{X_2,p_x} & \overline{X_2,p_y} & \overline{X_2,p_z} & & \end{array}\right] \\
&-i\sqrt{2}t_1t_2\beta\left[\begin{array}{ccccccc} & & \overline{X_1,p_x} & \overline{X_1,p_y} & \overline{X_1,p_z} & & \\ \underset{M_1,d_{x^2-y^2}}{\underline{\uparrow}} & \underset{M_1,d_{z^2}}{\underline{\uparrow\downarrow}} & & & & \underset{M_2,d_{x^2-y^2}}{\underline{\quad}} & \underset{M_2,d_{z^2}}{\underline{\uparrow}} \\ & & \overline{X_2,p_x} & \overline{X_2,p_y} & \overline{X_2,p_z} & & \end{array}\right]
\end{aligned}
$$

The $\uparrow$ and $\downarrow$ arrows here represent holes with spins sitting on the correspond orbitals of the sites labeled as $M_1, M_2, X_1, X_2$ on the $Z$ bond shown in Fig.1 of Ref. [28]. Similarly,

$$
\begin{aligned}
&T_{12}^{\text{eff}}|+1,0\rangle \\
=&d^\dagger_{M_1}\begin{pmatrix} d^\dagger_{M_1,z^2\uparrow} & d^\dagger_{M_1,z^2\downarrow} & 0 & 0 \\ 0 & 0 & d^\dagger_{M_1,z^2\uparrow} & d^\dagger_{M_1,z^2\downarrow} \\ -d^\dagger_{M_1,x^2-y^2\uparrow} & 0 & -d^\dagger_{M_1,x^2-y^2\downarrow} & 0 \\ 0 & -d^\dagger_{M_1,x^2-y^2\uparrow} & 0 & -d^\dagger_{M_1,x^2-y^2\downarrow} \end{pmatrix}\begin{pmatrix} 1 \\ 0 \\ 0 \\ 0 \end{pmatrix}|\text{vac}\rangle_{M_1} \\
&\otimes d^\dagger_{M_1}\begin{pmatrix} \mathbf{0} & 2t_1t_2\beta(iS^z) \\ -2t_1t_2\beta(iS^z) & \mathbf{0} \end{pmatrix}\begin{pmatrix} d^\dagger_{M_2,z^2\uparrow} & d^\dagger_{M_2,z^2\downarrow} & 0 & 0 \\ 0 & 0 & d^\dagger_{M_2,z^2\uparrow} & d^\dagger_{M_2,z^2\downarrow} \\ -d^\dagger_{M_2,x^2-y^2\uparrow} & 0 & -d^\dagger_{M_2,x^2-y^2\downarrow} & 0 \\ 0 & -d^\dagger_{M_2,x^2-y^2\uparrow} & 0 & -d^\dagger_{M_2,x^2-y^2\downarrow} \end{pmatrix}\begin{pmatrix} 0 \\ \frac{1}{\sqrt{2}} \\ \frac{1}{\sqrt{2}} \\ 0 \end{pmatrix}|\text{vac}\rangle_{M_2} \\
=&(d^\dagger_{M_1,x^2-y^2\uparrow}d^\dagger_{M_1,z^2\uparrow}-d^\dagger_{M_1,z^2\uparrow}d^\dagger_{M_1,x^2-y^2\uparrow})|\text{vac}\rangle_{M_1} \\
&\otimes\frac{it_1t_2\beta}{\sqrt{2}}(-d^\dagger_{M_1,x^2-y^2\uparrow}d^\dagger_{M_2,x^2-y^2\downarrow}+d^\dagger_{M_1,x^2-y^2\downarrow}d^\dagger_{M_2,x^2-y^2\uparrow}-d^\dagger_{M_1,z^2\uparrow}d^\dagger_{M_2,z^2\downarrow}+d^\dagger_{M_1,z^2\downarrow}d^\dagger_{M_2,z^2\uparrow})|\text{vac}\rangle_{M_2} \\
=&\quad i\sqrt{2}t_1t_2\beta\left[\begin{array}{ccccccc} & & \overline{X_1,p_x} & \overline{X_1,p_y} & \overline{X_1,p_z} & & \\ \underset{M_1,d_{x^2-y^2}}{\underline{\uparrow\downarrow}} & \underset{M_1,d_{z^2}}{\underline{\uparrow}} & & & & \underset{M_2,d_{x^2-y^2}}{\underline{\uparrow}} & \underset{M_2,d_{z^2}}{\underline{\quad}} \\ & & \overline{X_2,p_x} & \overline{X_2,p_y} & \overline{X_2,p_z} & & \end{array}\right] \\
&+i\sqrt{2}t_1t_2\beta\left[\begin{array}{ccccccc} & & \overline{X_1,p_x} & \overline{X_1,p_y} & \overline{X_1,p_z} & & \\ \underset{M_1,d_{x^2-y^2}}{\underline{\uparrow}} & \underset{M_1,d_{z^2}}{\underline{\uparrow\downarrow}} & & & & \underset{M_2,d_{x^2-y^2}}{\underline{\quad}} & \underset{M_2,d_{z^2}}{\underline{\uparrow}} \\ & & \overline{X_2,p_x} & \overline{X_2,p_y} & \overline{X_2,p_z} & & \end{array}\right]
\end{aligned}
$$

We refer to the energy spectra specified in Table I of the Supplementary Material of Ref. [34] to calculate $E_n - E_0$

between the excited and ground state energy for the $M_1, M_2, X_1, X_2$ system, and obtain

$$
\begin{aligned}
E_0 =& 2(U'_d - J_{H_d} + 2\varepsilon_M) + 2(3U_p + 12U'_p - 6J_{H_p} + 6\varepsilon_A) \\
E_n =& U_d + 2U'_d - J_{H_d} + 3\varepsilon_M + \varepsilon_M + 2(3U_p + 12U'_p - 6J_{H_p} + 6\varepsilon_A)
\end{aligned}
$$

This yields $E_n - E_0 = U_d - J_{H_d}$, where $U_d$ is the Hubbard repulsion on Ni $e_g$ orbitals, and $J_{H_d}$ is the Hund's coupling for the spin exchange and pair hopping within the $e_g$ orbitals.

The coupling strength of the nearest-neighbor spin interaction between $M_1$ and $M_2$ on the $Z$ bond of the honeycomb lattice is given by

$$
\langle +1, 0|H^{\text{eff}}|0, +1\rangle = -\sum_{n=n_1,n_2} \frac{\langle +1, 0|T_{12}^{\text{eff}\dagger}|n\rangle\langle n|T_{12}^{\text{eff}}|0, +1\rangle}{E_n - E_0} + \text{Conj.} = \frac{8t_1^2 t_2^2 \beta^2}{U_d - J_{H_d}} \tag{6}
$$

Note that $\langle +1, +1|H^{\text{eff}}|+1, +1\rangle = 0$ because the corresponding hopping is forbidden by the Hund's coupling through the same hopping path, so that

$$
K^z = -J^z_{\text{ind}} = -\frac{8t_1^2 t_2^2 \beta^2}{U_d - J_{H_d}} \tag{7}
$$

In addition to the upward one-hole process, we can also have a second one-hole process in which the hole originates from the following sequence: One hole from both $M_1$ and $M_2$ simultaneously jumps to $X_1(X_2)$ and $X_2(X_1)$, respectively, resulting in excited states. Consequently, the intermediate state features one hole on each of the $M_1, M_2, X_1$, and $X_2$ sites. The intermediate hopping matrix is altered accordingly as

$$
\begin{aligned}
T_{\text{I}}^{\text{eff}} =& p^\dagger_{X_1} \begin{pmatrix} t_1\mathbf{I} & -t_2\mathbf{I} \\ \mathbf{0} & \mathbf{0} \\ \mathbf{0} & \mathbf{0} \end{pmatrix} d_{M_1} \otimes p^\dagger_{X_2} \begin{pmatrix} -t_1\alpha\mathbf{I} & t_2\alpha\mathbf{I} \\ -t_1\beta(iS^z) & t_2\beta(iS^z) \\ t_1\beta(iS^y) & -t_2\beta(iS^y) \end{pmatrix} d_{M_2} \\
T_{\text{II}}^{\text{eff}} =& p^\dagger_{X_1} \begin{pmatrix} t_1\beta(iS^z) & t_2\beta(iS^z) \\ -t_1\alpha\mathbf{I} & -t_2\alpha\mathbf{I} \\ -t_1\beta(iS^x) & -t_2\beta(iS^x) \end{pmatrix} d_{M_2} \otimes p^\dagger_{X_2} \begin{pmatrix} \mathbf{0} & \mathbf{0} \\ t_1\mathbf{I} & t_2\mathbf{I} \\ \mathbf{0} & \mathbf{0} \end{pmatrix} d_{M_1}
\end{aligned}
$$

$T_{\text{I}}^{\text{eff}} + T_{\text{II}}^{\text{eff}\dagger}$ and $T_{\text{II}}^{\text{eff}} + T_{\text{I}}^{\text{eff}\dagger}$ work as perturbations to the on-site Hamiltonian of the local model containing $M_1, M_2, X_1, X_2$, to give rise to the effective spin model, which within the $S = 1$ subspace can be written as

$$
H^{\text{eff}} \sim -\sum_{\alpha\beta}\sum_{n\neq 0}\left(\frac{\langle\alpha|T_{\text{II}}^{\text{eff}\dagger}|n\rangle\langle n|T_{\text{I}}^{\text{eff}}|\beta\rangle}{E_n - E_0} + \frac{\langle\alpha|T_{\text{I}}^{\text{eff}\dagger}|n\rangle\langle n|T_{\text{II}}^{\text{eff}}|\beta\rangle}{E_n - E_0}\right)|\alpha\rangle\langle\beta| \tag{8}
$$

where, $|\alpha\rangle$ and $|\beta\rangle$, which run over $|0, +1\rangle$, $|+1, 0\rangle$, and $|+1, +1\rangle$ , are essential to calculate $J^z_{\text{ind}}$ and $K^z$. Specifically, we requires the excited states $T_{\text{I}}^{\text{eff}}|0, +1\rangle$, $T_{\text{II}}^{\text{eff}}|+1, 0\rangle$ (and their conjugate $T_{\text{II}}^{\text{eff}}|0, +1\rangle$, $T_{\text{I}}^{\text{eff}}|+1, 0\rangle$), $T_{\text{I}}^{\text{eff}}|+1, +1\rangle$, and $T_{\text{II}}^{\text{eff}}|+1, +1\rangle$. Eventually, the common intermediate states labeled as $n_1, n_2, n_3$ and $n_4$ contribute to the final energy

of spin superexchange, as shown below:

$$
\begin{aligned}
&T_{\mathrm{I}}^{\mathrm{eff}}|0,+1\rangle\\
=&p^{\dagger}_{X_1}\begin{pmatrix} t_1\mathbf{I} & -t_2\mathbf{I}\\ \mathbf{0} & \mathbf{0}\\ \mathbf{0} & \mathbf{0}\end{pmatrix}\begin{pmatrix} d^{\dagger}_{M_1,z^2\uparrow} & d^{\dagger}_{M_1,z^2\downarrow} & 0 & 0\\ 0 & 0 & d^{\dagger}_{M_1,z^2\uparrow} & d^{\dagger}_{M_1,z^2\downarrow}\\ -d^{\dagger}_{M_1,x^2-y^2\uparrow} & 0 & -d^{\dagger}_{M_1,x^2-y^2\downarrow} & 0\\ 0 & -d^{\dagger}_{M_1,x^2-y^2\uparrow} & 0 & -d^{\dagger}_{M_1,x^2-y^2\downarrow}\end{pmatrix}\begin{pmatrix}0\\ \frac{1}{\sqrt{2}}\\ \frac{1}{\sqrt{2}}\\ 0\end{pmatrix}|\mathrm{vac}\rangle_{M_1}\\
&\otimes p^{\dagger}_{X_2}\begin{pmatrix} -t_1\alpha\mathbf{I} & t_2\alpha\mathbf{I}\\ -t_1\beta(iS^z) & t_2\beta(iS^z)\\ t_1\beta(iS^y) & -t_2\beta(iS^y)\end{pmatrix}\begin{pmatrix} d^{\dagger}_{M_2,z^2\uparrow} & d^{\dagger}_{M_2,z^2\downarrow} & 0 & 0\\ 0 & 0 & d^{\dagger}_{M_2,z^2\uparrow} & d^{\dagger}_{M_2,z^2\downarrow}\\ -d^{\dagger}_{M_2,x^2-y^2\uparrow} & 0 & -d^{\dagger}_{M_2,x^2-y^2\downarrow} & 0\\ 0 & -d^{\dagger}_{M_2,x^2-y^2\uparrow} & 0 & -d^{\dagger}_{M_2,x^2-y^2\downarrow}\end{pmatrix}\begin{pmatrix}1\\0\\0\\0\end{pmatrix}|\mathrm{vac}\rangle_{M_2}\\
=&\frac{t_1}{\sqrt{2}}(p^{\dagger}_{X_1,x\uparrow}d^{\dagger}_{M_1,z^2\downarrow}+p^{\dagger}_{X_1,x\downarrow}d^{\dagger}_{M_1,z^2\uparrow}\\
&+p^{\dagger}_{X_1,x\uparrow}d^{\dagger}_{M_1,x^2-y^2\downarrow}+p^{\dagger}_{X_1,x\downarrow}d^{\dagger}_{M_1,x^2-y^2\uparrow})|\mathrm{vac}\rangle_{M_1,X_1}\\
\otimes&(-t_1\alpha p^{\dagger}_{X_2,x\uparrow}d^{\dagger}_{M_2,z^2\uparrow}-t_2\alpha p^{\dagger}_{X_2,x\uparrow}d^{\dagger}_{M_2,x^2-y^2\uparrow}\\
&-\frac{it_1\beta}{2}p^{\dagger}_{X_2,y\uparrow}d^{\dagger}_{M_2,z^2\uparrow}-\frac{it_2\beta}{2}p^{\dagger}_{X_2,y\uparrow}d^{\dagger}_{M_2,x^2-y^2\uparrow}\\
&-\frac{t_1\beta}{2}p^{\dagger}_{X_2,z\downarrow}d^{\dagger}_{M_2,z^2\uparrow}-\frac{t_2\beta}{2}p^{\dagger}_{X_2,z\downarrow}d^{\dagger}_{M_2,x^2-y^2\uparrow})|\mathrm{vac}\rangle_{M_2,X_2}
\end{aligned}
$$

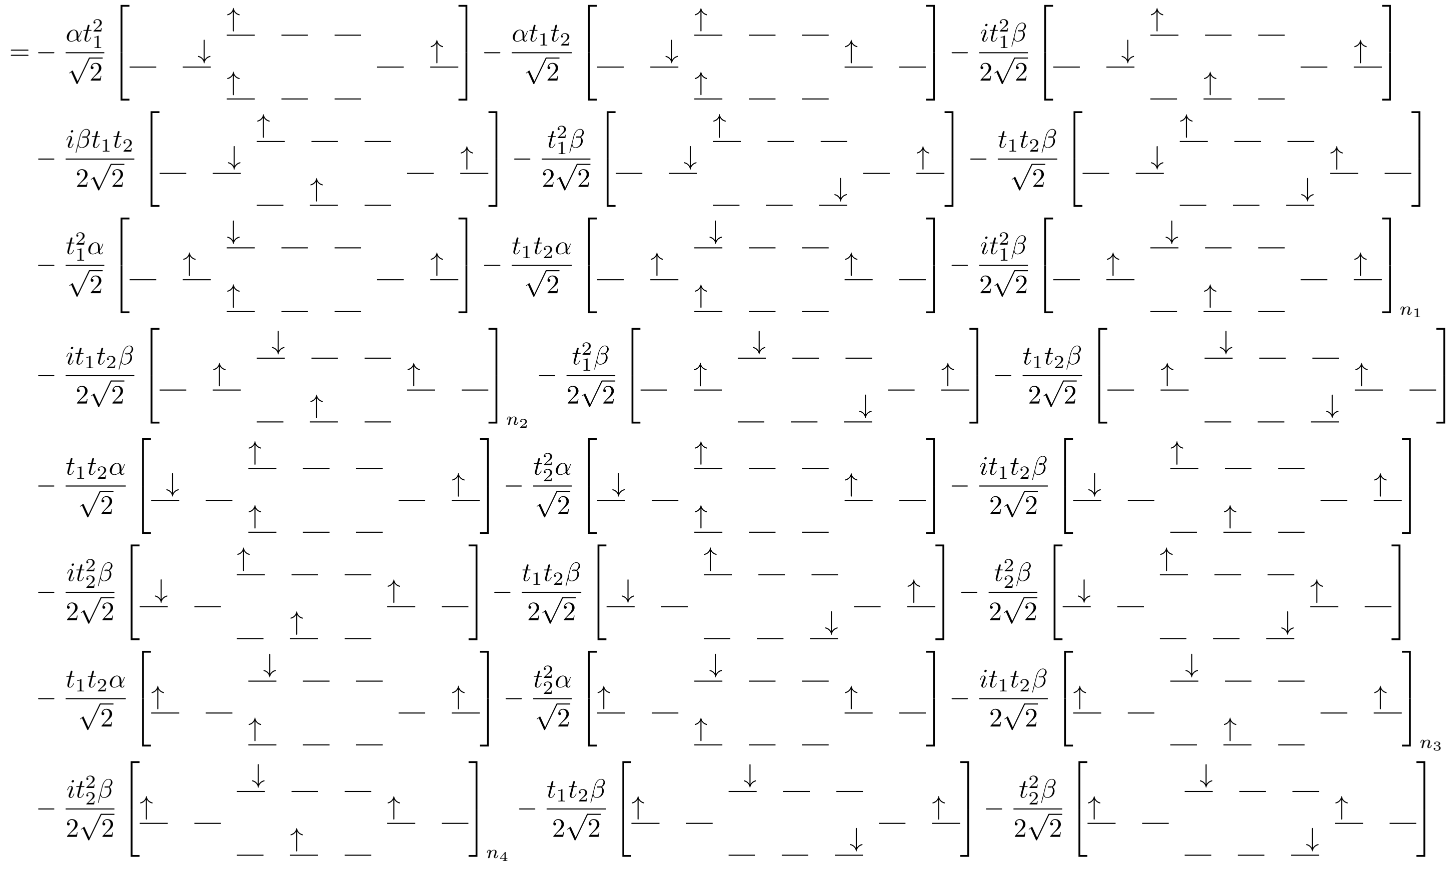

$$
\begin{aligned}
&T_{\mathrm{II}}^{\mathrm{eff}}|{+1},0\rangle \\
=&p^{\dagger}_{X_1}\begin{pmatrix}\beta t_1(iS^z) & \beta t_2(iS^z)\\ -\alpha t_1\mathbf{I} & -\alpha t_2\mathbf{I}\\ -\beta t_1(iS^x) & -\beta t_2(iS^x)\end{pmatrix}\begin{pmatrix} d^{\dagger}_{M_2,z^2\uparrow} & d^{\dagger}_{M_2,z^2\downarrow} & 0 & 0\\ 0 & 0 & d^{\dagger}_{M_2,z^2\uparrow} & d^{\dagger}_{M_2,z^2\downarrow}\\ -d^{\dagger}_{M_2,x^2-y^2\uparrow} & 0 & -d^{\dagger}_{M_2,x^2-y^2\downarrow} & 0\\ 0 & -d^{\dagger}_{M_2,x^2-y^2\uparrow} & 0 & -d^{\dagger}_{M_2,x^2-y^2\downarrow}\end{pmatrix}\begin{pmatrix}0\\ \frac{1}{\sqrt{2}}\\ \frac{1}{\sqrt{2}}\\ 0\end{pmatrix}|\mathrm{vac}\rangle_{M_2}\\
&\otimes p^{\dagger}_{X_2}\begin{pmatrix}\mathbf{0} & \mathbf{0}\\ t_1\mathbf{I} & t_2\mathbf{I}\\ \mathbf{0} & \mathbf{0}\end{pmatrix}\begin{pmatrix} d^{\dagger}_{M_1,z^2\uparrow} & d^{\dagger}_{M_1,z^2\downarrow} & 0 & 0\\ 0 & 0 & d^{\dagger}_{M_1,z^2\uparrow} & d^{\dagger}_{M_1,z^2\downarrow}\\ -d^{\dagger}_{M_1,x^2-y^2\uparrow} & 0 & -d^{\dagger}_{M_1,x^2-y^2\downarrow} & 0\\ 0 & -d^{\dagger}_{M_1,x^2-y^2\uparrow} & 0 & -d^{\dagger}_{M_1,x^2-y^2\downarrow}\end{pmatrix}\begin{pmatrix}1\\0\\0\\0\end{pmatrix}|\mathrm{vac}\rangle_{M_1}\\
=&(t_1p^{\dagger}_{X_2,y\uparrow}d^{\dagger}_{M_1,z^2\uparrow}-t_2p^{\dagger}_{X_2,y\uparrow}d^{\dagger}_{M_1,x^2-y^2\uparrow})|\mathrm{vac}\rangle_{M_1,X_2}\\
\otimes&\Big(\frac{it_1\beta}{2\sqrt{2}}p^{\dagger}_{X_1,x\uparrow}d^{\dagger}_{M_2,z^2\downarrow}-\frac{it_2\beta}{2\sqrt{2}}p^{\dagger}_{X_1,x\uparrow}d^{\dagger}_{M_2,x^2-y^2\downarrow}\\
&-\frac{it_1\beta}{2\sqrt{2}}p^{\dagger}_{X_1,x\downarrow}d^{\dagger}_{M_2,z^2\uparrow}+\frac{it_2\beta}{2\sqrt{2}}p^{\dagger}_{X_1,x\downarrow}d^{\dagger}_{M_2,x^2-y^2\uparrow}\\
&-\frac{t_1\alpha}{\sqrt{2}}p^{\dagger}_{X_1,y\uparrow}d^{\dagger}_{M_2,z^2\downarrow}+\frac{t_2\alpha}{\sqrt{2}}p^{\dagger}_{X_1,y\uparrow}d^{\dagger}_{M_2,x^2-y^2\downarrow}\\
&-\frac{t_1\alpha}{\sqrt{2}}p^{\dagger}_{X_1,y\downarrow}d^{\dagger}_{M_2,z^2\uparrow}+\frac{t_2\alpha}{\sqrt{2}}p^{\dagger}_{X_1,y\downarrow}d^{\dagger}_{M_2,x^2-y^2\uparrow}\\
&-\frac{it_1\beta}{2\sqrt{2}}p^{\dagger}_{X_1,z\uparrow}d^{\dagger}_{M_2,z^2\uparrow}+\frac{t_2\alpha}{\sqrt{2}}p^{\dagger}_{X_1,y\downarrow}d^{\dagger}_{M_2,x^2-y^2\uparrow}\\
&-\frac{it_1\beta}{2\sqrt{2}}p^{\dagger}_{X_1,z\uparrow}d^{\dagger}_{M_2,z^2\downarrow}+\frac{it_2\beta}{2\sqrt{2}}p^{\dagger}_{X_1,z\downarrow}d^{\dagger}_{M_2,x^2-y^2\downarrow}\Big)|\mathrm{vac}\rangle_{M_2,X_2}
\end{aligned}
$$

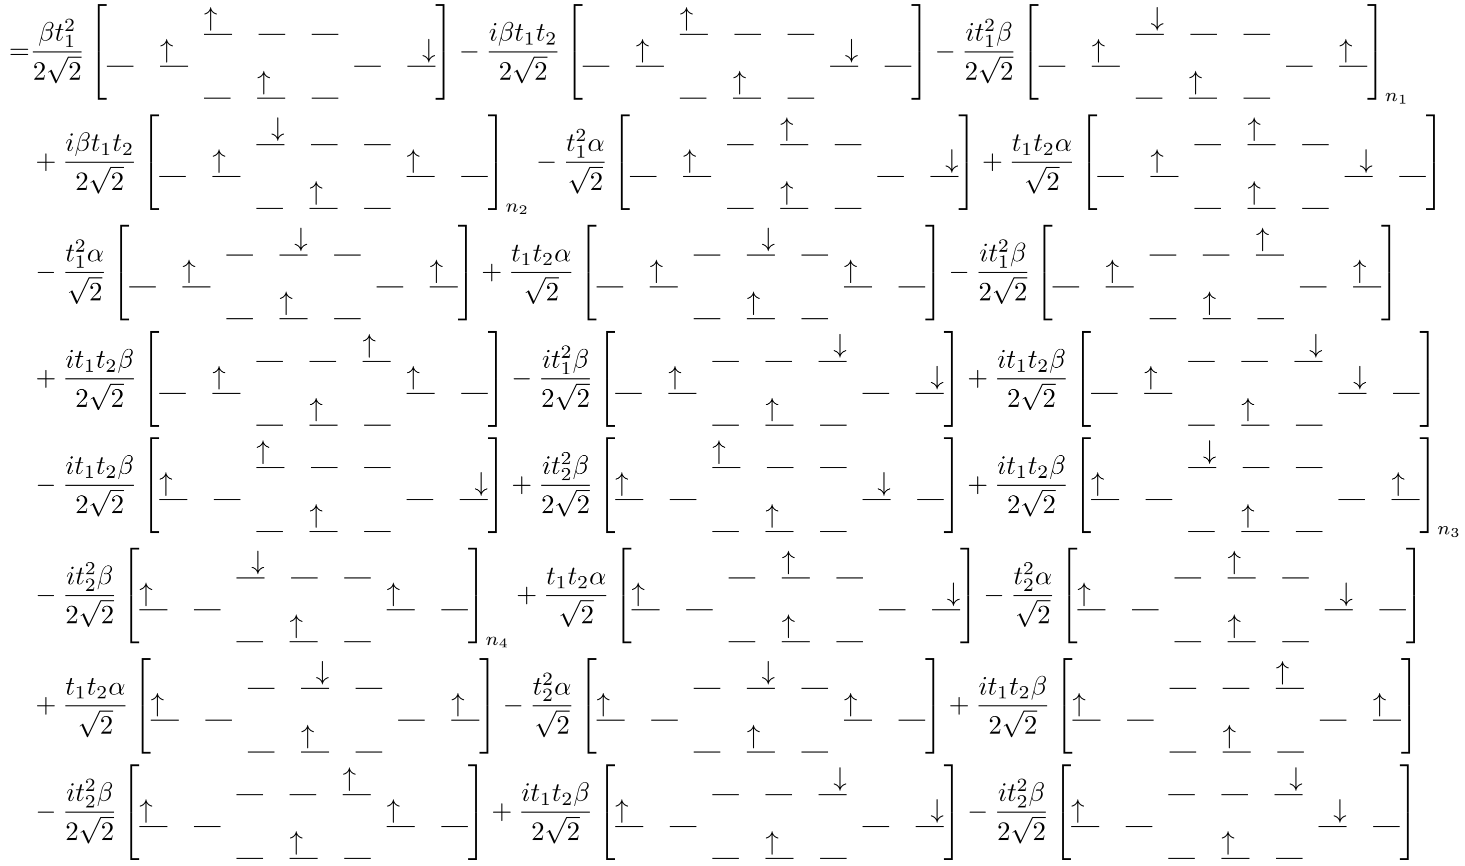

$$
\begin{aligned}
&T_{\mathrm{I}}^{\mathrm{eff}}|{+1},{+1}\rangle\\
=&p^{\dagger}_{X_1}\begin{pmatrix} t_1\mathbf{I} & -t_2\mathbf{I}\\ \mathbf{0} & \mathbf{0}\\ \mathbf{0} & \mathbf{0}\end{pmatrix}\begin{pmatrix} d^{\dagger}_{M_1,z^2\uparrow} & d^{\dagger}_{M_1,z^2\downarrow} & 0 & 0\\ 0 & 0 & d^{\dagger}_{M_1,z^2\uparrow} & d^{\dagger}_{M_1,z^2\downarrow}\\ -d^{\dagger}_{M_1,x^2-y^2\uparrow} & 0 & -d^{\dagger}_{M_1,x^2-y^2\downarrow} & 0\\ 0 & -d^{\dagger}_{M_1,x^2-y^2\uparrow} & 0 & -d^{\dagger}_{M_1,x^2-y^2\downarrow}\end{pmatrix}\begin{pmatrix}1\\0\\0\\0\end{pmatrix}|\mathrm{vac}\rangle_{M_1}\\
&\otimes p^{\dagger}_{X_2}\begin{pmatrix} -t_1\alpha\mathbf{I} & t_2\alpha\mathbf{I}\\ -t_1\beta(iS^z) & t_2\beta(iS^z)\\ t_1\beta(iS^y) & -t_2\beta(iS^y)\end{pmatrix}\begin{pmatrix} d^{\dagger}_{M_2,z^2\uparrow} & d^{\dagger}_{M_2,z^2\downarrow} & 0 & 0\\ 0 & 0 & d^{\dagger}_{M_2,z^2\uparrow} & d^{\dagger}_{M_2,z^2\downarrow}\\ -d^{\dagger}_{M_2,x^2-y^2\uparrow} & 0 & -d^{\dagger}_{M_2,x^2-y^2\downarrow} & 0\\ 0 & -d^{\dagger}_{M_2,x^2-y^2\uparrow} & 0 & -d^{\dagger}_{M_2,x^2-y^2\downarrow}\end{pmatrix}\begin{pmatrix}1\\0\\0\\0\end{pmatrix}|\mathrm{vac}\rangle_{M_2}\\
=&(t_1p^{\dagger}_{X_1,x\uparrow}d^{\dagger}_{M_1,z^2\uparrow}+t_2p^{\dagger}_{X_1,x\uparrow}d^{\dagger}_{M_1,x^2-y^2\uparrow})|\mathrm{vac}\rangle_{M_1,X_1}\\
\otimes&(-t_1\alpha p^{\dagger}_{X_2,x\uparrow}d^{\dagger}_{M_2,z^2\uparrow}-t_2\alpha p^{\dagger}_{X_2,x\uparrow}d^{\dagger}_{M_2,x^2-y^2\uparrow}-\frac{it_1\beta}{2}p^{\dagger}_{X_2,y\uparrow}d^{\dagger}_{M_2,z^2\uparrow}\\
&-\frac{it_2\beta}{2}p^{\dagger}_{X_2,y\uparrow}d^{\dagger}_{M_2,x^2-y^2\uparrow}-\frac{t_1\beta}{2}p^{\dagger}_{X_2,z\downarrow}d^{\dagger}_{M_2,z^2\uparrow}-\frac{t_2\beta}{2}p^{\dagger}_{X_2,z\downarrow}d^{\dagger}_{M_2,x^2-y^2\uparrow})|\mathrm{vac}\rangle_{M_2,X_2}\\
=&-\alpha t_1^2\begin{bmatrix} & & \underline{\uparrow} & \underline{\quad} & \underline{\quad} & & \\ \underline{\quad} & \underline{\uparrow} & & & & \underline{\quad} & \underline{\uparrow}\\ & & \underline{\uparrow} & \underline{\quad} & \underline{\quad} & & \end{bmatrix}-\alpha t_1t_2\begin{bmatrix} & & \underline{\uparrow} & \underline{\quad} & \underline{\quad} & & \\ \underline{\quad} & \underline{\uparrow} & & & & \underline{\uparrow} & \underline{\quad}\\ & & \underline{\uparrow} & \underline{\quad} & \underline{\quad} & & \end{bmatrix}-\frac{i\beta t_1^2}{2}\begin{bmatrix} & & \underline{\uparrow} & \underline{\quad} & \underline{\quad} & & \\ \underline{\quad} & \underline{\uparrow} & & & & \underline{\quad} & \underline{\uparrow}\\ & & \underline{\quad} & \underline{\uparrow} & \underline{\quad} & & \end{bmatrix}_{n_1}\\
&-\frac{i\beta t_1t_2}{2}\begin{bmatrix} & & \underline{\uparrow} & \underline{\quad} & \underline{\quad} & & \\ \underline{\quad} & \underline{\uparrow} & & & & \underline{\uparrow} & \underline{\quad}\\ & & \underline{\quad} & \underline{\uparrow} & \underline{\quad} & & \end{bmatrix}_{n_2}-\frac{\beta t_1^2}{2}\begin{bmatrix} & & \underline{\uparrow} & \underline{\quad} & \underline{\quad} & & \\ \underline{\quad} & \underline{\uparrow} & & & & \underline{\quad} & \underline{\uparrow}\\ & & \underline{\quad} & \underline{\quad} & \underline{\downarrow} & & \end{bmatrix}-\frac{\beta t_1t_2}{2}\begin{bmatrix} & & \underline{\uparrow} & \underline{\quad} & \underline{\quad} & & \\ \underline{\quad} & \underline{\uparrow} & & & & \underline{\uparrow} & \underline{\quad}\\ & & \underline{\quad} & \underline{\quad} & \underline{\downarrow} & & \end{bmatrix}\\
&-\alpha t_1t_2\begin{bmatrix} & & \underline{\uparrow} & \underline{\quad} & \underline{\quad} & & \\ \underline{\uparrow} & \underline{\quad} & & & & \underline{\quad} & \underline{\uparrow}\\ & & \underline{\uparrow} & \underline{\quad} & \underline{\quad} & & \end{bmatrix}-\alpha t_2^2\begin{bmatrix} & & \underline{\uparrow} & \underline{\quad} & \underline{\quad} & & \\ \underline{\uparrow} & \underline{\quad} & & & & \underline{\uparrow} & \underline{\quad}\\ & & \underline{\uparrow} & \underline{\quad} & \underline{\quad} & & \end{bmatrix}-\frac{i\beta t_1t_2}{2}\begin{bmatrix} & & \underline{\uparrow} & \underline{\quad} & \underline{\quad} & & \\ \underline{\uparrow} & \underline{\quad} & & & & \underline{\quad} & \underline{\uparrow}\\ & & \underline{\quad} & \underline{\uparrow} & \underline{\quad} & & \end{bmatrix}_{n_3}\\
&-\frac{i\beta t_2^2}{2}\begin{bmatrix} & & \underline{\uparrow} & \underline{\quad} & \underline{\quad} & & \\ \underline{\uparrow} & \underline{\quad} & & & & \underline{\uparrow} & \underline{\quad}\\ & & \underline{\quad} & \underline{\uparrow} & \underline{\quad} & & \end{bmatrix}_{n_4}-\frac{\beta t_1t_2}{2}\begin{bmatrix} & & \underline{\uparrow} & \underline{\quad} & \underline{\quad} & & \\ \underline{\uparrow} & \underline{\quad} & & & & \underline{\quad} & \underline{\uparrow}\\ & & \underline{\quad} & \underline{\quad} & \underline{\downarrow} & & \end{bmatrix}-\frac{\beta t_2^2}{2}\begin{bmatrix} & & \underline{\uparrow} & \underline{\quad} & \underline{\quad} & & \\ \underline{\uparrow} & \underline{\quad} & & & & \underline{\uparrow} & \underline{\quad}\\ & & \underline{\quad} & \underline{\quad} & \underline{\downarrow} & & \end{bmatrix}
\end{aligned}
$$

$$
\begin{aligned}
&T_{\mathrm{II}}^{\mathrm{eff}}|{+1},{+1}\rangle\\
=&p^{\dagger}_{X_1}\begin{pmatrix} \beta t_1(iS^z) & \beta t_2(iS^z)\\ -\alpha t_1\mathbf{I} & -\alpha t_2\mathbf{I}\\ -\beta t_1(iS^x) & -\beta t_2(iS^x)\end{pmatrix}\begin{pmatrix} d^{\dagger}_{M_2,z^2\uparrow} & d^{\dagger}_{M_2,z^2\downarrow} & 0 & 0\\ 0 & 0 & d^{\dagger}_{M_2,z^2\uparrow} & d^{\dagger}_{M_2,z^2\downarrow}\\ -d^{\dagger}_{M_2,x^2-y^2\uparrow} & 0 & -d^{\dagger}_{M_2,x^2-y^2\downarrow} & 0\\ 0 & -d^{\dagger}_{M_2,x^2-y^2\uparrow} & 0 & -d^{\dagger}_{M_2,x^2-y^2\downarrow}\end{pmatrix}\begin{pmatrix}1\\0\\0\\0\end{pmatrix}|\mathrm{vac}\rangle_{M_2}\\
&\otimes p^{\dagger}_{X_2}\begin{pmatrix} \mathbf{0} & \mathbf{0}\\ t_1\mathbf{I} & t_2\mathbf{I}\\ \mathbf{0} & \mathbf{0}\end{pmatrix}\begin{pmatrix} d^{\dagger}_{M_1,z^2\uparrow} & d^{\dagger}_{M_1,z^2\downarrow} & 0 & 0\\ 0 & 0 & d^{\dagger}_{M_1,z^2\uparrow} & d^{\dagger}_{M_1,z^2\downarrow}\\ -d^{\dagger}_{M_1,x^2-y^2\uparrow} & 0 & -d^{\dagger}_{M_1,x^2-y^2\downarrow} & 0\\ 0 & -d^{\dagger}_{M_1,x^2-y^2\uparrow} & 0 & -d^{\dagger}_{M_1,x^2-y^2\downarrow}\end{pmatrix}\begin{pmatrix}1\\0\\0\\0\end{pmatrix}|\mathrm{vac}\rangle_{M_1}\\
=&(t_1p^{\dagger}_{X_2,y\uparrow}d^{\dagger}_{M_1,z^2\uparrow}-t_2p^{\dagger}_{X_2,y\uparrow}d^{\dagger}_{M_1,x^2-y^2\uparrow})|\mathrm{vac}\rangle_{M_1,X_2}\\
\otimes&(\frac{it_1\beta}{2}p^{\dagger}_{X_1,x\uparrow}d^{\dagger}_{M_2,z^2\uparrow}-\frac{it_2\beta}{2}p^{\dagger}_{X_1,x\uparrow}d^{\dagger}_{M_2,x^2-y^2\uparrow}\\
&-\alpha t_1p^{\dagger}_{X_1,y\uparrow}d^{\dagger}_{M_2,z^2\uparrow}+\alpha t_2p^{\dagger}_{X_1,y\uparrow}d^{\dagger}_{M_2,x^2-y^2\uparrow}\\
&-\frac{it_1\beta}{2}p^{\dagger}_{X_1,z\downarrow}d^{\dagger}_{M_2,z^2\uparrow}+\frac{it_2\beta}{2}p^{\dagger}_{X_1,z\downarrow}d^{\dagger}_{M_2,x^2-y^2\uparrow})
\end{aligned}
$$

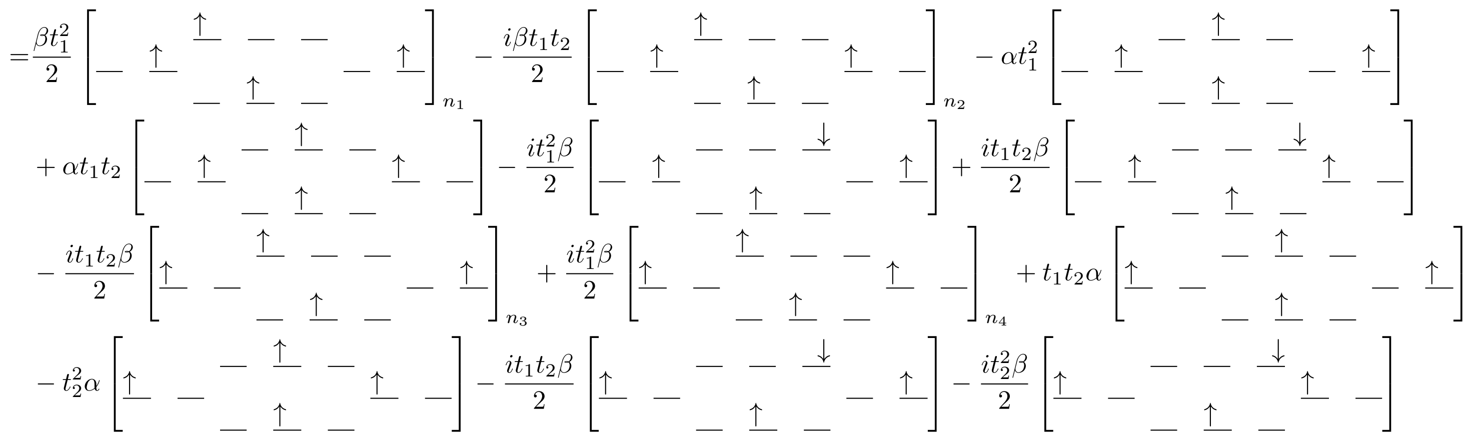

Moreover, the energy of the excited state is

$$
\begin{aligned}
E_0 =& 2(U'_d - J_{H_d} + 2\varepsilon_d) + 2(3U_p + 12U'_p - 6J_{H_p} + 6\varepsilon_p) \\
E_n =& 2(U'_d - J_{H_d} + 2\varepsilon_d) + 2(3U_p + 12U'_p - 6J_{H_p} + 6\varepsilon_p)
\end{aligned}
$$

So that we have $\Delta E_n \equiv E_n - E_0 = 2U_d + 2U'_d + 2\varepsilon_d - 2U_p - 8U'_p + 4J_{H_p} - 2\varepsilon_p$. Then the energy from the second hopping single-hole process is

$$
\begin{aligned}
\langle +1, 0|H^{\rm eff}|0, +1\rangle =& -\sum_{n=n_1\cdots n_4} \frac{\langle +1, 0|T_{\rm II}^{\rm eff\dagger}|n\rangle\langle n|T_{\rm I}^{\rm eff}|0, +1\rangle}{E_n - E_0} + {\rm Conj.} \\
=& -\frac{\beta^2(t_1^2 - t_2^2)^2}{4\Delta E_n}
\end{aligned}
$$

For the second hopping path $\langle +1, +1|H^{\rm eff}|+1, +1\rangle$ is non-zero. Since the derivation is very similar to that for the upward one-hole process, we write down the final result.

$$
\begin{aligned}
\langle +1, +1|H^{\rm eff}|+1, +1\rangle =& -\sum_{n=n_1\cdots n_4} \frac{\langle +1, +1|T_{\rm II}^{\rm eff\dagger}|n\rangle\langle n|T_{\rm I}^{\rm eff}|+1, +1\rangle}{E_n - E_0} + {\rm Conj.} \\
=& \frac{\beta^2(t_1^2 - t_2^2)^2}{2\Delta E_n}
\end{aligned}
$$

In short, the two different single-hole processes contribute to the Heisenberg term with energies

$$
\begin{aligned}
J^z_{\rm ind} &= -\frac{\beta^2(t_1^2 - t_2^2)^2}{4\Delta E_n} + \frac{8\beta^2 t_1^2 t_2^2}{U_d - J_{H_d}} \\
K^z_{\rm ind} &= \frac{3\beta^2(t_1^2 - t_2^2)^2}{4\Delta E_n} - \frac{8\beta^2 t_1^2 t_2^2}{U_p - J_{H_d}}
\end{aligned}
$$

where $t_1$, $t_2$ and $t_3$ are represented by the Slater-Koster parameters [35], so that $t_1 = \frac{\sqrt{3}}{2}t_{pd\sigma}$, $t_2 = \frac{1}{2}t_{pd\sigma}$ and $t_3 = t_{pd\sigma}$, which we have qualitatively confirmed through our DFT simulations. Therefore, $J^z_{\rm ind}$ and $K^z_{\rm ind}$ are given by

$$
\begin{aligned}
J^z_{\rm ind} &= -\frac{\beta^2 t^4_{pd\sigma}}{2}[\frac{1}{8\Delta E_n} - \frac{3}{U_d - J_{H_d}}] \\
K^z_{\rm ind} &= \frac{\beta^2 t^4_{pd\sigma}}{2}[\frac{3}{8\Delta E_n} - \frac{3}{U_p - J_{H_d}}]
\end{aligned}
$$

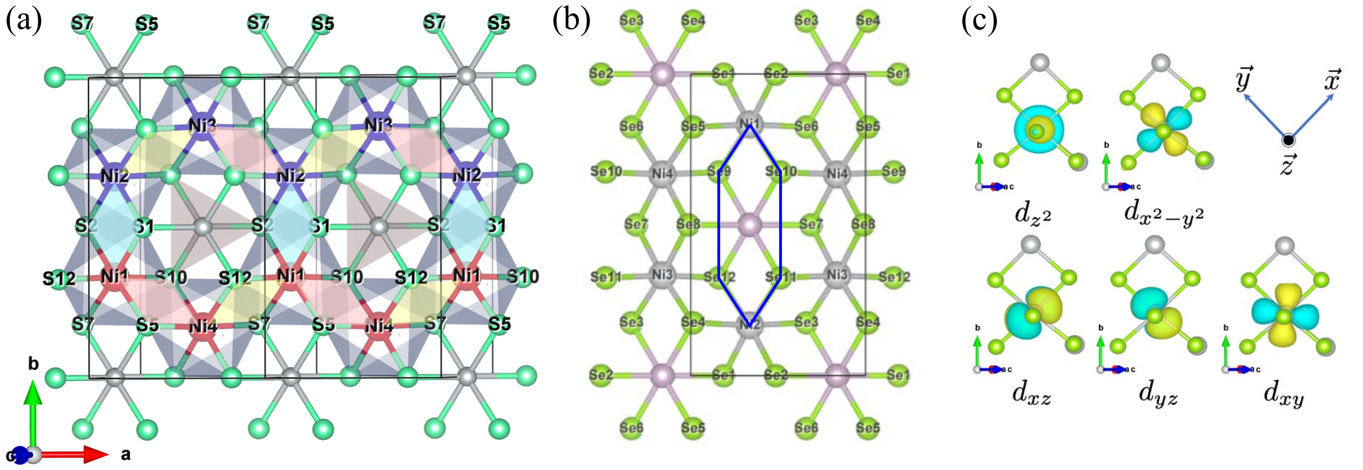


FIG. S2. (a) The coordination number of Ni and the ligand in each unit cell is noted. The hopping integrals of overlapped orbitals within each $M$–$X$–$M$ path are indicated by yellow, blue, and red colors. Correspondingly, the hopping integrals for different orbital overlaps are detailed in the subsequent tables, using the same color scheme. (b) The coordination number of Ni and the ligand in each unit cell regarding $M$–$X$–$X$–$M$ hopping path for $J_3$ is noted. (c) $3d$ orbitals of Ni atoms with fully filled $t_{2g}$ orbitals in the bottom row and half-filled $e_g$ orbitals in the top row, which are aligned in accord with the global coordinate axis $\{\vec{x}, \vec{y}, \vec{z}\}$.

In the Mott-Hubbard region, $\Delta_{pd} \gg U_d$ where $\Delta_{pd} = \varepsilon_d - \varepsilon_p$ is the charge transfer energy, so that $\frac{3}{8\Delta E_n}$ will be much smaller than $\frac{3}{U_p - J_{H_d}}$ and the effective Kitaev term is approximately given by

$$K^z \approx \frac{3}{2}\beta^2 t_{pd\sigma}^4 \frac{1}{U_d - J_{H_d}} = \frac{1}{6}\lambda_p^2 t_{pd\sigma}^4 \left(\frac{1}{\Delta_{pd} - \lambda_p} + \frac{2}{\Delta_{pd} + \frac{\lambda_p}{2}}\right)^2 \frac{1}{(2\Delta_{pd} - \lambda_p)^2 (U_d - J_{H_d})}$$

where $\beta = \frac{-\alpha\lambda_p}{2\Delta_{pd} - \lambda_p}$ and $\alpha = \frac{1}{3}\left(\frac{1}{\Delta_{pd} - \lambda_p} + \frac{2}{\Delta_{pd} + \frac{\lambda_p}{2}}\right)$. It can be further simplified as

$$K^z \approx \frac{3}{2} \frac{t_{pd\sigma}^4 \lambda_p^2}{(2\Delta_{pd}^2 - \lambda_p \Delta_{pd} - \lambda_p^2)^2 (U_d - J_{H_d})} \tag{9}$$

Note that the single-hole process also contributes to the scaling of $J_{\mathrm{ind}}^z$ with $\lambda_p^2$. However, as analyzed in Ref. [26], the two-hole process also contributes to the indirect spin coupling, where the Heisenberg terms originating from the two-hole process do not scale with $\lambda_p$ and are always present. In our work, it is exciting to see the emergence of a finite $K^\gamma$ term when sulfur is replaced with selenium at the ligand site. This effectively turns on $\lambda_p$ through chemical replacement and triggers the activation of $K^\gamma$. Subsequently, we employ DFT approach to further estimate the strength of these coupling terms.

It should be noted that the ligand-mediated *ferromagnetic* $J_1$ might be counterbalanced by the *antiferromagnetic* spin coupling through direct spin exchange between the two nearest-neighbor Ni sites. Suggesting that by carefully balancing these two sources of $J_1$, it may be possible to ensure that $K^\gamma$ prevails over $J_1$ [26].

## IV. ESTIMATING HOPPING INTEGRALS

Hopping integrals involve overlaps of the nearest-neighbor Ni-Ni and Ni-ligand orbitals. The relevant Ni and ligand sites are marked in Fig.S2a. Notably, direct hopping between the two nearest-neighbor Ni $d$ orbitals is significantly smaller than the hopping integral through the metal-ligand path, implying that the $ferromagnetic$ $J_1$ resulting from $M$–$X$–$M$ super-exchange, is likely to dominate the $J_1$ coupling. The Slater-Koster formulation remains applicable even in the presence of lattice distortions and deviations from perfect cubic symmetry. This can also be seen from the forms of the following matrices (in meV), where $t_1 = (\sqrt{3}/2)t_{pd\sigma}$, $t_2 = t_{pd\sigma}/2$, $t_3 = t_{pd\sigma}$, so that $t_1^2 + t_2^2 = t_3^2$ is satisfied.

| | $Ni^{[4]}_{d_{xz}}$ | $Ni^{[4]}_{d_{yz}}$ | $Ni^{[4]}_{d_{xy}}$ | $Ni^{[4]}_{d_{z^2}}$ | $Ni^{[4]}_{d_{x^2-y^2}}$ |
|---|---|---|---|---|---|
| $Ni^{[1]}_{d_{xz}}$ | 0.023468 | 0.053161 | 0.045329 | 0.009898 | −0.002753 |
| $Ni^{[1]}_{d_{yz}}$ | 0.053156 | −0.128763 | 0.045345 | −0.033301 | 0.044219 |
| $Ni^{[1]}_{d_{xy}}$ | 0.045321 | 0.045341 | 0.047318 | −0.039824 | −0.015393 |
| $Ni^{[1]}_{d_{z^2}}$ | 0.0099 | −0.033331 | −0.039835 | −0.07604 | −0.128173 |
| $Ni^{[1]}_{d_{x^2-y^2}}$ | −0.002737 | 0.044207 | −0.015378 | −0.128166 | 0.05259 |

| | $S^{[5]}_{p_z}$ | $S^{[5]}_{p_x}$ | $S^{[5]}_{p_y}$ | $S^{[10]}_{p_z}$ | $S^{[10]}_{p_x}$ | $S^{[10]}_{p_y}$ |
|---|---|---|---|---|---|---|
| $Ni^{[1]}_{d_{xz}}$ | −0.082735 | −0.052471 | −0.053731 | 0.259228 | 0.403792 | 0.018614 |
| $Ni^{[1]}_{d_{yz}}$ | 0.446153 | −0.029634 | 0.279638 | −0.172423 | −0.008672 | 0.451249 |
| $Ni^{[1]}_{d_{xy}}$ | −0.009226 | 0.323036 | 0.287027 | −0.011071 | 0.077331 | −0.028629 |
| $Ni^{[1]}_{d_{z^2}}$ | −0.174698 | −0.037365 | 0.465108 | −0.83269 | 0.187089 | −0.234777 |
| $Ni^{[1]}_{d_{x^2-y^2}}$ | −0.082479 | −0.320284 | 0.644185 | −0.070539 | 0.016275 | 0.004265 |

| | $Ni^{[2]}_{d_{xz}}$ | $Ni^{[2]}_{d_{yz}}$ | $Ni^{[2]}_{d_{xy}}$ | $Ni^{[2]}_{d_{z^2}}$ | $Ni^{[2]}_{d_{x^2-y^2}}$ |
|---|---|---|---|---|---|
| $Ni^{[1]}_{d_{xz}}$ | 0.039515 | 0.039399 | −0.000993 | −0.040001 | −0.03191 |
| $Ni^{[1]}_{d_{yz}}$ | 0.039404 | 0.067383 | −0.020803 | 0.02829 | −0.03827 |
| $Ni^{[1]}_{d_{xy}}$ | −0.003536 | −0.019406 | −0.148827 | 0.072411 | 0.00298 |
| $Ni^{[1]}_{d_{z^2}}$ | −0.036818 | 0.026025 | 0.064647 | 0.084436 | −0.022859 |
| $Ni^{[1]}_{d_{x^2-y^2}}$ | −0.031609 | −0.039603 | 0.003012 | −0.025596 | −0.14141 |

| | $S^{[1]}_{p_z}$ | $S^{[1]}_{p_x}$ | $S^{[1]}_{p_y}$ | $S^{[2]}_{p_z}$ | $S^{[2]}_{p_x}$ | $S^{[2]}_{p_y}$ |
|---|---|---|---|---|---|---|
| $Ni^{[1]}_{d_{xz}}$ | −0.370658 | 0.197502 | 0.102628 | 0.048056 | 0.095032 | 0.020653 |
| $Ni^{[1]}_{d_{yz}}$ | −0.080103 | 0.082813 | −0.066056 | −0.376119 | 0.000798 | −0.226503 |
| $Ni^{[1]}_{d_{xy}}$ | 0.085254 | 0.304562 | −0.392903 | 0.009155 | −0.397331 | −0.366815 |
| $Ni^{[1]}_{d_{z^2}}$ | −0.207556 | −0.34145 | −0.128883 | 0.207545 | −0.007637 | −0.364925 |
| $Ni^{[1]}_{d_{x^2-y^2}}$ | 0.120089 | 0.716313 | 0.304398 | 0.146929 | 0.259216 | −0.702369 |

| | $Ni^{[2]}_{d_{xz}}$ | $Ni^{[2]}_{d_{yz}}$ | $Ni^{[2]}_{d_{xy}}$ | $Ni^{[2]}_{d_{z^2}}$ | $Ni^{[2]}_{d_{x^2-y^2}}$ |
|---|---|---|---|---|---|
| $Ni^{[3]}_{d_{xz}}$ | −0.160248 | −0.008411 | 0.010227 | 0.025854 | 0.074161 |
| $Ni^{[3]}_{d_{yz}}$ | −0.00842 | 0.041882 | −0.051349 | −0.005601 | 0.029124 |
| $Ni^{[3]}_{d_{xy}}$ | 0.010232 | −0.051347 | 0.067121 | 0.030295 | −0.015455 |
| $Ni^{[3]}_{d_{z^2}}$ | 0.025831 | −0.005609 | 0.030276 | −0.05275 | 0.064774 |
| $Ni^{[3]}_{d_{x^2-y^2}}$ | 0.074173 | 0.02914 | −0.015462 | 0.064763 | −0.014789 |

| | $S^{[12]}_{p_z}$ | $S^{[12]}_{p_x}$ | $S^{[12]}_{p_y}$ | $S^{[7]}_{p_z}$ | $S^{[7]}_{p_x}$ | $S^{[7]}_{p_y}$ |
|---|---|---|---|---|---|---|
| $Ni^{[1]}_{d_{xz}}$ | −0.248987 | −0.44285 | −0.005137 | 0.448194 | −0.268976 | −0.084016 |
| $Ni^{[1]}_{d_{yz}}$ | 0.18692 | −0.032438 | −0.412238 | 0.070703 | −0.059909 | 0.041782 |
| $Ni^{[1]}_{d_{xy}}$ | −0.035726 | −0.040165 | 0.038776 | −0.044707 | −0.322133 | 0.366062 |
| $Ni^{[1]}_{d_{z^2}}$ | 0.83262 | −0.283765 | 0.098123 | 0.174717 | 0.450964 | 0.119826 |
| $Ni^{[1]}_{d_{x^2-y^2}}$ | −0.061834 | 0.034251 | −0.05283 | −0.070005 | −0.657889 | −0.183702 |

As discussed in the main text that an analysis [30] of perturbation theory shows that the energy scale of $J_3 \sim t^4_{pd\sigma} t^2_{pp\sigma}/\Delta^4_{pd}(U_d - J_{H_d})$ is substantial because $t_{pp\sigma}$ hopping integral between Se $p$ orbitals along the hopping path inducing $J_3$ is sizable, this can also be seen from the following matrix of relevant ligand sites marked in Fig.S2b.

| | $Se^{[10]}_{p_z}$ | $Se^{[10]}_{p_x}$ | $Se^{[10]}_{p_y}$ |
|---|---|---|---|
| $Se^{[11]}_{p_z}$ | −0.118257 | −0.297302 | −0.017736 |
| $Se^{[11]}_{p_x}$ | −0.0899 | 0.342878 | 0.557928 |
| $Se^{[11]}_{p_y}$ | 0.310929 | −1.252491 | 0.100972 |

Along with the hopping matrices of relevant Ni and ligand sites also marked in Fig. S2b.

| | $Se^{[10]}_{p_z}$ | $Se^{[10]}_{p_x}$ | $Se^{[10]}_{p_y}$ |
|---|---|---|---|
| $Ni^{[1]}_{d_{xz}}$ | −0.076045 | −0.047263 | −0.056877 |
| $Ni^{[1]}_{d_{yz}}$ | 0.349887 | −0.038887 | 0.24568 |
| $Ni^{[1]}_{d_{xy}}$ | −0.030009 | 0.246244 | 0.280109 |
| $Ni^{[1]}_{d_{z^2}}$ | −0.145899 | −0.045642 | 0.363902 |
| $Ni^{[1]}_{d_{x^2-y^2}}$ | −0.108546 | −0.254549 | 0.517069 |

| | $Se^{[11]}_{p_z}$ | $Se^{[11]}_{p_x}$ | $Se^{[11]}_{p_y}$ |
|---|---|---|---|
| $Ni^{[2]}_{d_{xz}}$ | −0.38996 | 0.29890 | 0.082179 |
| $Ni^{[2]}_{d_{yz}}$ | −0.04978 | 0.062939 | −0.039100 |
| $Ni^{[2]}_{d_{xy}}$ | 0.06173 | 0.28670 | −0.28869 |
| $Ni^{[2]}_{d_{z^2}}$ | −0.16896 | −0.46192 | −0.095608 |
| $Ni^{[2]}_{d_{x^2-y^2}}$ | 0.12917 | 0.71874 | 0.23865 |

[1] Pierre Hohenberg and Walter Kohn. Inhomogeneous electron gas. *Physical Review*, 136(3B):B864, 1964.
[2] Georg Kresse and Jürgen Furthmüller. Efficient iterative schemes for ab initio total-energy calculations using a plane-wave basis set. *Physical Review B*, 54(16):11169, 1996.
[3] Georg Kresse and Daniel Joubert. From ultrasoft pseudopotentials to the projector augmented-wave method. *Physical Review B*, 59(3):1758, 1999.
[4] John P Perdew, Kieron Burke, and Matthias Ernzerhof. Generalized gradient approximation made simple. *Physical Review letters*, 77(18):3865, 1996.
[5] Vladimir I. Anisimov, Jan Zaanen, and Ole K. Andersen. Band theory and Mott insulators: Hubbard U instead of Stoner I. *Physical Review B*, 44:943, 1991.
[6] Vladimir I Anisimov, F Aryasetiawan, and A I Lichtenstein. First-principles calculations of the electronic structure and spectra of strongly correlated systems: the LDA + U method. *Journal of Physics: Condensed Matter*, 9(4):767, 1997.
[7] Stefan Grimme, Jens Antony, Stephan Ehrlich, and Helge Krieg. A consistent and accurate *abinitio* parametrization of density functional dispersion correction (DFT-D) for the 94 elements H-Pu. *The Journal of Chemical Physics*, 132(15):154104, 2010.
[8] Hendrik J. Monkhorst and James D. Pack. Special points for Brillouin-zone integrations. *Physical Review B*, 13:5188, 1976.
[9] A Il Liechtenstein, MI Katsnelson, VP Antropov, and VA Gubanov. Local spin density functional approach to the theory of exchange interactions in ferromagnetic metals and alloys. *Journal of Magnetism and Magnetic Materials*, 67(1):65–74, 1987.
[10] Xu He, Nicole Helbig, Matthieu J Verstraete, and Eric Bousquet. TB2J: A python package for computing magnetic interaction parameters. *Computer Physics Communications*, 264:107938, 2021.
[11] Nicola Marzari and David Vanderbilt. Maximally localized generalized Wannier functions for composite energy bands. *Physical Review B*, 56(20):12847, 1997.
[12] Soner Steiner, Sergii Khmelevskyi, Martijn Marsmann, and Georg Kresse. Calculation of the magnetic anisotropy with projected-augmented-wave methodology and the case study of disordered $\mathrm{fe}_{1-x}\mathrm{co}_x$ alloys. *Phys. Rev. B*, 93:224425, Jun 2016.
[13] K. W. Plumb, J. P. Clancy, L. J. Sandilands, V. Vijay Shankar, Y. F. Hu, K. S. Burch, Hae-Young Kee, and Young-June Kim. $\alpha-\mathrm{RuCl}_3$: A spin-orbit assisted Mott insulator on a honeycomb lattice. *Physical Review B*, 90:041112, 2014.
[14] Heung-Sik Kim, Kristjan Haule, and David Vanderbilt. Mott Metal-Insulator Transitions in Pressurized Layered Trichalcogenides. *Physical Review Letters*, 123:236401, 2019.
[15] Hualei Sun, Liang Qiu, Yifeng Han, Enkui Yi, Junlong Li, Mengwu Huo, Chaoxin Huang, Hui Liu, Manrong Li, Weiliang Wang, Dao-Xin Yao, Benjamin A. Frandsen, Bing Shen, Yusheng Hou, and Meng Wang. Coexistence of zigzag antiferromagnetic order and superconductivity in compressed $\mathrm{NiPSe}_3$. *Materials Today Physics*, 36:101188, 2023.
[16] D. Lançon, R. A. Ewings, T. Guidi, F. Formisano, and A. R. Wildes. Magnetic exchange parameters and anisotropy of the quasi-two-dimensional antiferromagnet $\mathrm{NiPS}_3$. *Physical Review B*, 98:134414, 2018.
[17] A. Scheie, Pyeongjae Park, J. W. Villanova, G. E. Granroth, C. L. Sarkis, Hao Zhang, M. B. Stone, Je-Geun Park, S. Okamoto, T. Berlijn, and D. A. Tennant. Spin wave Hamiltonian and anomalous scattering in $\mathrm{NiPS}_3$. *Physical Review B*, 108:104402, 2023.
[18] Carmine Autieri, Giuseppe Cuono, Canio Noce, Milosz Rybak, Kamila M. Kotur, Cliò Efthimia Agrapidis, Krzysztof Wohlfeld, and Magdalena Birowska. Limited Ferromagnetic Interactions in Monolayers of $\mathrm{MPS}_3$ (M = Mn and Ni). *The Journal of Physical Chemistry C*, 126(15):6791–6802, 2022.
[19] Bheema Lingam Chittari, Youngju Park, Dongkyu Lee, Moonsup Han, Allan H. MacDonald, Euyheon Hwang, and Jeil Jung. Electronic and magnetic properties of single-layer $M\mathrm{P}X_3$ metal phosphorous trichalcogenides. *Physical Review B*, 94:184428, 2016.
[20] Yuhao Gu, Qiang Zhang, Congcong Le, Yinxiang Li, Tao Xiang, and Jiangping Hu. Ni-based transition metal trichalcogenide monolayer: A strongly correlated quadruple-layer graphene. *Physical Review B*, 100:165405, 2019.
[21] N. Bazazzadeh, M. Hamdi, F. Haddadi, A. Khavasi, A. Sadeghi, and S. M. Mohseni. Symmetry enhanced spin-Nernst effect in honeycomb antiferromagnetic transition metal trichalcogenide monolayers. *Physical Review B*, 103:014425, 2021.
[22] N. Bazazzadeh, M. Hamdi, S. Park, A. Khavasi, S. M. Mohseni, and A. Sadeghi. Magnetoelastic coupling enabled tunability of magnon spin current generation in two-dimensional antiferromagnets. *Physical Review B*, 104:L180402, 2021.
[23] Rabindra Basnet, Kamila M. Kotur, Milosz Rybak, Cory Stephenson, Samuel Bishop, Carmine Autieri, Magdalena Birowska, and Jin Hu. Controlling magnetic exchange and anisotropy by nonmagnetic ligand substitution in layered $M\mathrm{P}X_3$ ($M$ = Ni, Mn; $X$ = S, Se). *Physical Review Research*, 4:023256, 2022.
[24] Rajan Plumley, Sougata Mardanya, Cheng Peng, Johannes Nokelainen, Tadesse Assefa, Lingjia Shen, Nicholas Burdet, Zach Porter, Alexander Petsch, Aidan Israelski, Hongwei Chen, Jun Sik Lee, Sophie Morley, Sujoy Roy, Gilberto Fabbris, Elizabeth Blackburn, Adrian Feiguin, Arun Bansil, Wei-Sheng Lee, Aaron Lindenberg, Sugata Chowdhury, Mike Dunne, and Joshua J. Turner. 3D Heisenberg universality in the Van der Waals antiferromagnet $\mathrm{NiPS}_3$. *arXiv e-prints*, page arXiv:2310.07948, 2023.
[25] G. Jackeli and G. Khaliullin. Mott Insulators in the Strong Spin-Orbit Coupling Limit: From Heisenberg to a Quantum Compass and Kitaev Models. *Physical Review Letters*, 102:017205, 2009.
[26] P. Peter Stavropoulos, D. Pereira, and Hae-Young Kee. Microscopic Mechanism for a Higher-Spin Kitaev Model. *Physical*

*Review Letters*, 123:037203, 2019.
[27] Jeffrey G. Rau, Eric Kin-Ho Lee, and Hae-Young Kee. Generic Spin Model for the Honeycomb Iridates beyond the Kitaev Limit. *Physical Review Letters*, 112:077204, 2014.
[28] P. Peter Stavropoulos, Xiaoyu Liu, and Hae-Young Kee. Magnetic anisotropy in spin-3/2 with heavy ligand in honeycomb Mott insulators: Application to $CrI_3$. *Physical Review Research*, 3:013216, 2021.
[29] Changsong Xu, Junsheng Feng, Hongjun Xiang, and Laurent Bellaiche1. Interplay between Kitaev interaction and single ion anisotropy in ferromagnetic $CrI_3$ and $CrGeTe_3$ monolayers. *npj Computational Materials*, 4, 2018.
[30] Stephen M Winter. Magnetic couplings in edge-sharing high-spin $d^7$ compounds. *Journal of Physics: Materials*, 5(4):045003, 2022.
[31] Meng-Chien Wang and Ching-Ray Chang. Goodenough-Kanamori-Anderson Rules in $CrI_3/MoTe_2/CrI_3$ Van der Waals Heterostructure. *Journal of The Electrochemical Society*, 169(5):053507, 2022.
[32] Chaebin Kim, Heung-Sik Kim, and Je-Geun Park. Spin-orbital entangled state and realization of Kitaev physics in $3d$ cobalt compounds: a progress report. *Journal of Physics: Condensed Matter*, 34(2):023001, 2021.
[33] Swati Chaudhary, Alon Ron, David Hsieh, and Gil Refael. Controlling ligand-mediated exchange interactions in periodically driven magnetic materials. *arXiv e-prints*, page arXiv:2009.00813, 2020.
[34] P. Peter Stavropoulos, D. Pereira, and Hae-Young Kee. Microscopic Mechanism for a Higher-Spin Kitaev Model. *Physical Review Letters*, 123:037203, 2019.
[35] J. C. Slater and G. F. Koster. Simplified LCAO Method for the Periodic Potential Problem. *Physical Review*, 94:1498–1524, 1954.
